# Supplementary material for: Estimating Peer Effects Using Partial Network Data
Source: arXiv:2509.08145 source file (2025-09-09)
Supplement: Supplementary file 9 [file letter_appendix_2.tex]

\section*{Referees' Appendix}

In this note, we sketch a proof showing that the variance of the moment function of our SGMM estimator is smaller than the variance of an alternative moment function that would only use two draws.

Following the discussion at the beginning of Section 3 of the manuscript, another alternative to our SGMM is to directly correct the bias of the initial function \( \dot{\mathbf{m}}_m (\boldsymbol{\theta}) = \dot{\mathbf{Z}}_m^{\prime} \dot{\boldsymbol{\varepsilon}}_m(\boldsymbol{\theta}) \) (see Page 15).

In this case, an (unfeasible) de-biased moment function would be:
\begin{align}
    &\dot{\mathbf m}_m (\boldsymbol{\theta}) - \mathbb{E}[\dot{\mathbf m}_m (\boldsymbol{\theta})|\mathbf{X}_m, \mathcal{A}_m, \dot{\mathbf{G}}_m, \mathbf{G}_m] = \nonumber\\
    &\dot{\mathbf Z}_m^{\prime}(\mathbf I_m - \alpha \dot{\mathbf G}_m ) \big[\mathbf y_m - (\mathbf I_m - \alpha_0 \mathbf G_m )^{-1}(c_0\mathbf{1}_m + \mathbf X_m\boldsymbol{\beta}_0 + {\mathbf G}_m\mathbf X_m\boldsymbol{\gamma}_0)\big].\nonumber
\end{align}
The feasible equivalent of this moment function is thus:
\begin{equation} \label{eq:moment:2simu}\tag{1}
\dot{\mathbf Z}_m^{\prime}(\mathbf I_m - \alpha \dot{\mathbf G}_m ) \big[\mathbf y_m - (\mathbf I_m - \alpha \ddot{\mathbf G}_m )^{-1}(c\mathbf{1}_m + \mathbf X_m\boldsymbol{\beta} + \ddot{\mathbf G}_m\mathbf X_m\boldsymbol{\gamma})\big].
\end{equation}
While both moment functions in Theorem 1 and in (1) lead to consistent estimators, it can be shown that the one in Theorem 1 is more efficient because its variance is lower. The intuition is as follows.

In general, bias correction is associated with a loss of efficiency. With \( \dot{\mathbf{m}}_m (\boldsymbol{\theta}) \), we mechanically correct both the bias stemming from the dependence between \( \dot{\mathbf{Z}}_m \) and \( \dot{\boldsymbol{\varepsilon}}_m(\boldsymbol{\theta}_0) \), as well as the bias due to the fact that \( \dot{\boldsymbol{\varepsilon}}_m(\boldsymbol{\theta}_0) \) is not centered. In contrast, our proposed moment function (see Theorem 1) does not suffer from the first bias (since we use different draws for the instruments and the covariates), and we only correct for the second bias.

More formally, note that both moment functions have the form \(\dot{\mathbf Z}_m^{\prime}\mathbf u_m\) and \(\dot{\mathbf Z}_m^{\prime}\tilde{\mathbf u}_m\), where \(\mathbf u_m\) and \(\tilde{\mathbf u}_m\) are the terms that post-multiply \(\dot{\mathbf Z}_m^{\prime}\) in the moment function in Theorem 1, and (1), respectively. Although \(\mathbf u_m\) and \(\tilde{\mathbf u}_m\) have different expressions, they share the same distribution. Indeed, \(\mathbf u_m\) can be written as a function of \(\ddot{\mathbf G}_m\) and \(\dddot{\mathbf G}_m\), whereas \(\tilde{\mathbf u}_m\) can be written as the same function of \(\dot{\mathbf G}_m\) and \(\ddot{\mathbf G}_m\). Since the simulated networks have the same distribution, it follows that \(\mathbf u_m\) and \(\tilde{\mathbf u}_m\) also have the same distribution.

We aim to compare the variance of \(\dot{\mathbf Z}_m^{\prime}\mathbf u_m\) to the variance of \(\dot{\mathbf Z}_m^{\prime}\tilde{\mathbf u}_m\) in a situation where \(\mathbf u_m\) and \(\tilde{\mathbf u}_m\) have the same distribution, \(\tilde{\mathbf u}_m\) is correlated with \(\dot{\mathbf Z}\), and \(\mathbf u_m\) is independent of \(\dot{\mathbf Z}\), conditional on \(\mathbf{X}_m\) and \(\mathcal{A}_m\). Indeed, \(\dot{\mathbf Z}\) and \(\tilde{\mathbf u}_m\) are correlated because they depend on the same simulated network \(\dot{\mathbf G}_m\).

To simplify the comparison of the variances of \(\dot{\mathbf Z}_m^{\prime}\mathbf u_m\) and \(\dot{\mathbf Z}_m^{\prime}\tilde{\mathbf u}_m\), we assume that \(\dot{\mathbf Z}_m\), \(\mathbf u_m\), and \(\tilde{\mathbf u}_m\) are scalars. (It is possible to generalize the result by applying what follows to each entry of the variances, but the notation would become cumbersome.) Let \(\mathbb{V}_1\) and \(\mathbb{V}_2\) be the variances of \(\dot{\mathbf Z}_m^{\prime}\mathbf u_m\) and \(\dot{\mathbf Z}_m^{\prime}\tilde{\mathbf u}_m\), respectively, conditional on \(\mathbf{X}_m\) and \(\mathcal{A}_m\). We have:
\begin{align*}
    \mathbb{V}_2 - \mathbb{V}_1 &= \mathbb{E}(\dot{\mathbf Z}_m^2\tilde{\mathbf u}_m^2|\mathbf{X}_m, \mathcal{A}_m) -  \mathbb{E}(\dot{\mathbf Z}_m^2\mathbf u_m^2|\mathbf{X}_m, \mathcal{A}_m),\\
    \mathbb{V}_2 - \mathbb{V}_1 &= \mathbb{E}(\dot{\mathbf Z}_m^2\tilde{\mathbf u}_m^2|\mathbf{X}_m, \mathcal{A}_m) -  \mathbb{E}(\dot{\mathbf Z}_m^2|\mathbf{X}_m, \mathcal{A}_m)\mathbb{E}(\mathbf u_m^2|\mathbf{X}_m, \mathcal{A}_m),\\
    \mathbb{V}_2 - \mathbb{V}_1 &= \mathbb{E}(\dot{\mathbf Z}_m^2\tilde{\mathbf u}_m^2|\mathbf{X}_m, \mathcal{A}_m) -  \mathbb{E}(\dot{\mathbf Z}_m^2|\mathbf{X}_m, \mathcal{A}_m)\mathbb{E}(\tilde{\mathbf u}_m^2|\mathbf{X}_m, \mathcal{A}_m),\\
    \mathbb{V}_2 - \mathbb{V}_1 &= \operatorname{Cov}(\dot{\mathbf Z}_m^2, ~\tilde{\mathbf u}_m^2|\mathbf{X}_m, \mathcal{A}_m).
\end{align*}
In the third equality, we replace 
\(\mathbb{E}(\mathbf{u}_m^2 \mid \mathbf{X}_m, \mathcal{A}_m)\) 
with 
\(\mathbb{E}(\tilde{\mathbf{u}}_m^2 \mid \mathbf{X}_m, \mathcal{A}_m)\) 
because \(\mathbf{u}_m\) and \(\tilde{\mathbf{u}}_m\) share the same distribution. 
Thus, the moment function with two simulated networks performs better if 
\(\dot{\mathbf{Z}}_m^2\) and \(\tilde{\mathbf{u}}_m^2\) are positively correlated, 
conditional on \(\mathbf{X}_m\) and \(\mathcal{A}_m\). 
This is straightforward to see when there are no contextual effects, 
as both \(\dot{\mathbf{Z}}_m\) and \(\tilde{\mathbf{u}}_m\) are linear in \(\dot{\mathbf{G}}_m\). 
Moreover, \(\dot{\mathbf{Z}}_m^2\) and \(\tilde{\mathbf{u}}_m^2\) remain positively correlated 
regardless of the sign of \(\alpha\).
