# Supplementary material for: Estimating Peer Effects Using Partial Network Data
Source: arXiv:2509.08145 source file (2025-09-09)
Supplement: Supplementary file 11 [file appendix_proof-bkp.tex]

\section{Appendix -- GMM estimator: assumptions and proofs}\label{sec:appendix_proofs}

Consider the following regularity assumptions.

\begin{assumption}\label{as:regularity}
$\boldsymbol{\rho}_0\in int(\mathcal{R})$ and $\boldsymbol{\theta}_0\in int(\Theta)$, where $\mathcal{R}$ and $\Theta$ are both compact subsets of the Euclidean space.
\end{assumption}

\begin{assumption}\label{as:nonsingular}
For all $r=1,...,R$, $s=1,...,S$, and $t=1,...,T$, $(\mathbf{I}-\alpha \dot{\mathbf{G}}^{r})$, $(\mathbf{I}-\alpha \ddot{\mathbf{G}}^{s})$ and $(\mathbf{I}-\alpha \dddot{\mathbf{G}}^{t})$ are non-singular
\end{assumption}
In particular, when $\mathbf{G}$ is row-normalized (so $\dot{\mathbf{G}}^{r}$, $\ddot{\mathbf{G}}^{s}$, and $\dddot{\mathbf{G}}^{t}$ are also row-normalized), Assumption \ref{as:alpha} implies Assumption \ref{as:nonsingular}.

We consider an objective function for the GMM estimator of the usual form: $$\textstyle\left(\frac{1}{M}\sum_i \mathbf{m}_i(\boldsymbol{\theta})\right)'\mathbf{W}_N\left(\frac{1}{N}\sum_i \mathbf{m}_i(\boldsymbol{\theta})\right),$$
where $\mathbf{m}_i(\boldsymbol{\theta})$ is the moment function.
\begin{assumption}\label{as:weigth}
$\mathbf{W}_N$ is symmetric and positive definite with $\mathbf{W}_N\rightarrow_p\mathbf{W}_0$ for $\mathbf{W}_0$ also symmetric and positive definite.
\end{assumption}

\subsection{Proof of Theorem \ref{prop:non_observed}}

The proof proceeds in three stages. First, we establish consistency and discuss the identification and numerical implementation. Second, we show how the estimator can be written as a sequential m-estimator and establish asymptotic normality. Third, we show how to estimate the asymptotic variance, without relying on the asymptotic normality.

\subsubsection{Validity of the moment condition and consistency}
Let $$\textstyle\mathbf{m}_i(\boldsymbol{\theta})=\frac{1}{RST}\sum_r\sum_s\sum_t\dot{\mathbf{Z}}_i^{(r)\prime}(\mathbf{I}-\alpha\dddot{\mathbf{G}}^{(t)})_i\left(\mathbf{y}-(\mathbf{I}-\alpha\ddot{\mathbf{G}}^{(s)})^{-1}\ddot{\mathbf{V}}^{(s)}\tilde{\boldsymbol{\theta}}\right)$$

We will show that, by construction, we have: $\textstyle\plim\mathbb{E}\left(\mathbf{m}_i(\boldsymbol{\theta})\right)=\mathbf{0}$ for any finite $S$ and $T$, where $\plim$ is the probability limit.

To see why, lets substitute $\mathbf{y}=(\mathbf{I}-\alpha\mathbf{G})^{-1}(\mathbf{V}\tilde{\boldsymbol{\theta}}+\boldsymbol{\varepsilon})$ in the moment function. We have:
\begin{eqnarray*}
\textstyle\mathbf{m}_i(\boldsymbol{\theta})&=&\textstyle\frac{1}{RST}\sum_r\sum_s\sum_t \dot{\mathbf{Z}}_i^{(r)\prime}(\mathbf{I}-\alpha\dddot{\mathbf{G}}^{(t)})_i\left[(\mathbf{I}-\alpha\mathbf{G})^{-1}\mathbf{V}-(\mathbf{I}-\alpha\ddot{\mathbf{G}}^{(s)})^{-1}\ddot{\mathbf{V}}^{(s)}\right]\tilde{\boldsymbol{\theta}}\\
&+&\textstyle\frac{1}{RS}\sum_r\sum_s \dot{\mathbf{Z}}_i^{(r)\prime}(\mathbf{I}-\alpha\dddot{\mathbf{G}}^{(t)})_i(\mathbf{I}-\alpha\mathbf{G})^{-1}\boldsymbol{\varepsilon}
\end{eqnarray*}

Consider the second term first. For any $r,~s,~t$, we have:
$$\textstyle
\mathbb{E}\left(\dot{\mathbf{Z}}_i^{(r)\prime}(\mathbf{I}-\alpha\dddot{\mathbf{G}}^{(t)})_i(\mathbf{I}-\alpha\mathbf{G})^{-1}\boldsymbol{\varepsilon}\right)=\mathbf{0},
$$
directly from Assumption \ref{as:exonet} and the specification of the network formation process (see Assumption \ref{as:partial}).

Consider now the first term. We need:
$$\textstyle
\plim \mathbb{E}\left[\dot{\mathbf{Z}}_i^{(r)\prime}(\mathbf{I}-\alpha\dddot{\mathbf{G}}^{(t)})_i\left[(\mathbf{I}-\alpha\mathbf{G})^{-1}\mathbf{V}-(\mathbf{I}-\alpha\ddot{\mathbf{G}}^{(s)})^{-1}\ddot{\mathbf{V}}^{(s)}\right]\tilde{\boldsymbol{\theta}}\right]=\mathbf{0}.
$$

\noindent Note that, for N fixed, $\mathbf{G}$, $\dot{\mathbf{G}}^{(r)}$, $\ddot{\mathbf{G}}^{(s)}$, and $\dddot{\mathbf{G}}^{(t)}$ have a finite number of possible realizations. Thus, $\textstyle\mathbb{E}\left[\dot{\mathbf{Z}}_i^{(s)\prime}(\mathbf{I}-\alpha\dddot{\mathbf{G}}^{(t)})_i(\mathbf{I}-\alpha\mathbf{G})^{-1}\mathbf{V}\tilde{\boldsymbol{\theta}}\right]$ can be written as a continuous function of $P$, the distribution of the adjacency matrix, and $\hat{P}$, a consistent estimator of that distribution.\footnote{The function would essentially composed of summations and products of terms depending on $P$ and $\hat{P}$.} Analogously, $\mathbb{E}\left[\dot{\mathbf{Z}}_i^{(s)\prime}(\mathbf{I}-\alpha\dddot{\mathbf{G}}^{(t)})_i(\mathbf{I}-\alpha\ddot{\mathbf{G}}^{(s)})^{-1}\ddot{\mathbf{V}}^{(s)}\tilde{\boldsymbol{\theta}}\right]$ also can be written as a same function with the difference that $P$ is replaced by $\hat{P}$. As both functions are continuous and since $\hat{P}$ converges in probability to $P$ (see Assumption \ref{as:partial}), their limits are obtained by replacing $\hat{P}$ by $P$ and then equal. As such, we have:
$$
\plim \mathbb{E}\left[\dot{\mathbf{Z}}_i^{(s)\prime}(\mathbf{I}-\alpha\dddot{\mathbf{G}}^{(t)})_i(\mathbf{I}-\alpha\mathbf{G})^{-1}\mathbf{V}\tilde{\boldsymbol{\theta}}\right]=\plim \mathbb{E}\left[\dot{\mathbf{Z}}_i^{(s)\prime}(\mathbf{I}-\alpha\dddot{\mathbf{G}}^{(t)})_i(\mathbf{I}-\alpha\ddot{\mathbf{G}}^{(s)})^{-1}\ddot{\mathbf{V}}^{(s)}\tilde{\boldsymbol{\theta}}\right].
$$

\noindent The GMM estimator
$$\textstyle
\hat{\boldsymbol{\theta}}=\arg\max \left(\frac{1}{N}\sum_i\mathbf{m}_i(\boldsymbol{\theta})\right)'\mathbf{W}_N\left(\frac{1}{N}\sum_i\mathbf{m}_i(\boldsymbol{\theta})\right)
$$
is therefore consistent under Assumptions \ref{as:manymarkets}-\ref{as:weigth} and an identification condition, which we now discuss.

\subsubsection{Concentration and Identification\label{app:ident}}
While the GMM estimator could be solved numerically, it is helpful to concentrate the objective function around $\alpha$.
Let $\textstyle\mathbf{R}(\alpha)=\frac{1}{RST}\sum_r\sum_s\sum_t\dot{\mathbf{Z}}^{(s)\prime}(\mathbf{I}-\alpha\dddot{\mathbf{G}}^{(t)})(\mathbf{I}-\alpha\ddot{\mathbf{G}}^{(s)})^{-1}\ddot{\mathbf{V}}^{(s)}$ and $\textstyle\mathbf{D}(\alpha)=\frac{1}{RST}\sum_r\sum_s\sum_t\dot{\mathbf{Z}}^{(s)\prime}(\mathbf{I}-\alpha\dddot{\mathbf{G}}^{(t)})$ so that $\textstyle\frac{1}{N}\sum_i\mathbf{m}_i(\boldsymbol{\theta})=\mathbf{D}(\alpha)\mathbf{y}-\mathbf{R}(\alpha)\tilde{\boldsymbol{\theta}}$.

The gradient of the objective function with respect to $\textstyle\tilde{\boldsymbol{\theta}}$ is:
$$
\textstyle-2\left(\frac{1}{N}\mathbf{D}(\alpha)\mathbf{y}-\mathbf{R}(\alpha)\tilde{\boldsymbol{\theta}}\right)'\mathbf{W}_N\mathbf{R(\alpha)}.
$$
The hessian is therefore: $\mathbf{R}'(\alpha)\mathbf{W}_N\mathbf{R(\alpha)}$ which is semi-positive definite. Hence, the following assumption ensures identification of $\tilde{\boldsymbol{\theta}}$, conditional on $\alpha$.

\begin{assumption}\label{as:convex}
$\mathbf{R}'(\alpha)\mathbf{W}_N\mathbf{R(\alpha)}$ is non-singular for all $\alpha$.
\end{assumption}
\noindent A sufficient condition is that $\mathbf{R}'(\alpha)$ has full rank, for all $\alpha$.\\
Under Assumption \ref{as:convex}, the estimator of $\tilde{\boldsymbol{\theta}}$ conditionally on $\alpha$ is\\ $\hat{\tilde{\boldsymbol{\theta}}}(\alpha)=(\mathbf{R}'(\alpha)\mathbf{W}_N\mathbf{R(\alpha)})^{-1}\mathbf{R}'(\alpha)\mathbf{W}_N\mathbf{D}(\alpha)\mathbf{y}$.\\
The objective function can then be concentrated around $\alpha$, as 
$$\textstyle
\left(\frac{1}{N}\mathbf{D}(\alpha)\mathbf{y}-\mathbf{R}(\alpha)\hat{\tilde{\boldsymbol{\theta}}}(\alpha)\right)'\mathbf{W}_N\left(\frac{1}{N}\mathbf{D}(\alpha)\mathbf{y}-\mathbf{R}(\alpha)\hat{\tilde{\boldsymbol{\theta}}}(\alpha)\right).
$$
While we cannot easily ensure that this function is globally convex in $\alpha$, the behavior of the function is easy to study since $\alpha$ is uni-dimensional and has a bounded support (see Assumption \ref{as:alpha}). Note that numerically minimizing the concentrated objective function implicitly checks Assumption \ref{as:convex}. Our final assumption ensures identification of $\alpha$.
\begin{assumption}\label{as:globalmin}
The concentrated objective function admits an interior global minimum.
\end{assumption}

We now turn to the asymptotic distribution of our estimator.

\subsubsection{Asymptotic Normality}
The challenge in showing the asymptotic normality of our estimator lies in the fact that we use a sequential estimation strategy.

Here, we assume that the model can be written as a sequential m-estimator. If the first stage estimator $\hat{\boldsymbol{\rho}}$ is an M-estimator, then it verifies the first-order conditions:
\begin{equation}\label{eq:dq1}
    \frac{1}{M}\sum_{m = 1}^M  \dfrac{\partial Q_{1,m}(\hat{\boldsymbol{\rho}})}{\partial  \boldsymbol{\rho}} = 0,
\end{equation} for some function $Q_{1,m}$. We assume that $Q_{1,m}(\boldsymbol{\rho})$ is twice continuously differentiable in $\boldsymbol{\rho}$. Note that even if the observational unit of the first stage is at the pair level, it is always possible to take the sum or the average of the moment condition at the pair pair level to produce a moment condition at the group level as in (\ref{eq:dq1}).

Consider now the second stage, i.e. our SGMM estimator, and the associated (computationally unfeasible) moment function:
\begin{equation}\label{eq:expectedmoment}
\mathbb{E}_{\dot{\mathbf{G}},\ddot{\mathbf{G}},\dddot{\mathbf{G}}|\hat{\boldsymbol{\rho}}}\left\{\dot{\mathbf{Z}}^{(r)\prime}_i\left[(\mathbf{I}-\alpha\dddot{\mathbf{G}}^{(t)})_i\left(\mathbf{y}-(\mathbf{I}-\alpha\ddot{\mathbf{G}}^{(s)})^{-1}\ddot{\mathbf{V}}^{(s)}\tilde{\boldsymbol{\theta}}\right)\right]\right\},
\end{equation}
which can be written as:
$$
\sum_{\dot{\mathbf{G}},\ddot{\mathbf{G}},\dddot{\mathbf{G}}} \dot{\mathbf{Z}}^{(r)\prime}_i\left[(\mathbf{I}-\alpha\dddot{\mathbf{G}}^{(t)})_i\left(\mathbf{y}-(\mathbf{I}-\alpha\ddot{\mathbf{G}}^{(s)})^{-1}\ddot{\mathbf{V}}^{(s)}\tilde{\boldsymbol{\theta}}\right)\right]\mathbb{P}(\dot{\mathbf{G}}|\hat{\boldsymbol{\rho}})\mathbb{P}(\ddot{\mathbf{G}}|\hat{\boldsymbol{\rho}})\mathbb{P}(\dddot{\mathbf{G}}|\hat{\boldsymbol{\rho}})
$$
As $R,S,T\rightarrow\infty$, the simulated moment function converges a.s. to the above expectation by a LLN.

Under the network formation specification (\ref{eq:gennetfor}), the GMM based on (\ref{eq:expectedmoment}) can be written as a m-estimator, twice continuously differentiable in $\mathbf{\rho}$ and $\mathbf{\theta}$:
\begin{equation}
    \label{eq:dq2}\frac{1}{M}\sum_{m=1}^M  \dfrac{\partial Q_{2,m}(\hat{\boldsymbol{\theta}}, \hat{\boldsymbol{\rho}})}{\partial  \boldsymbol{\theta}} = 0,
\end{equation}

Asymptotic normality therefore follows directly from standard results for sequential m-estimators, see e.g. \cite{cameron2005microeconometrics}, Section 6.6. We therefore have:
$$\sqrt{M}(\hat{\boldsymbol{\theta}} - \boldsymbol{\theta}_0) \overset{d}{\to} N(0, \boldsymbol{\Sigma}_0),$$

\noindent where $\boldsymbol{\Sigma}_0 = \plim \boldsymbol{\Sigma}_N$ and $\boldsymbol{\Sigma}_N = \Var(\sqrt{M}\hat{\boldsymbol{\theta}})$.

%We can then study the asymptotic of $\hat{\boldsymbol{\theta}}$ and $\hat{\boldsymbol{\rho}}$ jointly since they are both M-estimators \cite[see][]{cameron2005microeconometrics}. Under regulatory conditions that will hold in our case, $\left(\hat{\boldsymbol{\theta}}^{\prime}, \hat{\boldsymbol{\rho}}^{\prime}\right)^{\prime}$ is root-$M$ consistent and has a normal distribution asymptotically. In particular, we have

\subsubsection{Variance Estimation}
We now present a simple approach to estimate $\boldsymbol{\Sigma}_0$. Our approach does not rely on the asymptotic normality and takes into account the uncertainty related to the estimation at the first stage.

\noindent  Taking the first derivative of the objective function at the second stage (for finite $R$,$S$,$T$ and conditional on $\hat{\mathbf{\rho}}$) with respect to $\boldsymbol{\theta}$, we have:
$$
\dfrac{1}{N}\sum_i\frac{\partial\mathbf{m}_i^{\hat{P}}(\boldsymbol{\theta})^{\prime}}{\partial\boldsymbol{\theta}}\mathbf{W}_N\dfrac{1}{N}\sum_i\mathbf{m}_i^{\hat{P}}(\boldsymbol{\theta})=\mathbf{0}.
$$
By applying the mean value theorem to $\frac{1}{N}\sum_i\mathbf{m}_i^{\hat{P}}(\boldsymbol{\theta})$, we have:
$$\textstyle\sqrt{M}(\hat{\boldsymbol{\theta}}-\boldsymbol{\theta}_0)=-\left[\dfrac{1}{N}\sum_i\frac{\partial\mathbf{m}_i^{\hat{P}}(\hat{\boldsymbol{\theta}})^{\prime}}{\partial\boldsymbol{\theta}} \mathbf{W}_N \frac{1}{N}\sum_i\frac{\partial\mathbf{m}_i^{\hat{P}}({\boldsymbol{\theta}^*})}{\partial\boldsymbol{\theta}^{\prime}}\right]^{-1}\frac{1}{N}\sum_i\frac{\partial\mathbf{m}_i^{\hat{P}}(\hat{\boldsymbol{\theta}})^{\prime}}{\partial\boldsymbol{\theta}} \mathbf{W}_N\frac{\sqrt{M}}{N}\sum_i\mathbf{m}_i^{\hat{P}}(\boldsymbol{\theta}_0),   $$
where $\boldsymbol{\theta}^*$ is some point between $\hat{\boldsymbol{\theta}}$ and $\boldsymbol{\theta}_0$.  \\
Let $\textstyle\mathbf{H}_N = \left[\dfrac{1}{N}\sum_i\frac{\partial\mathbf{m}_i^{\hat{P}}(\hat{\boldsymbol{\theta}})^{\prime}}{\partial\boldsymbol{\theta}} \mathbf{W}_N \frac{1}{N}\sum_i\frac{\partial\mathbf{m}_i^{\hat{P}}({\boldsymbol{\theta}^*})}{\partial\boldsymbol{\theta}^{\prime}}\right]^{-1}\frac{1}{N}\sum_i\frac{\partial\mathbf{m}_i^{\hat{P}}(\hat{\boldsymbol{\theta}})^{\prime}}{\partial\boldsymbol{\theta}} \mathbf{W}_N$ and let $\mathbf{H}_0 = \plim \mathbf{H}_N$.\\
We have $$\textstyle\sqrt{M}(\hat{\boldsymbol{\theta}}-\boldsymbol{\theta}_0)=-\mathbf{H}_N\frac{\sqrt{M}}{N}\sum_i\mathbf{m}_i^{\hat{P}}(\boldsymbol{\theta}_0).$$
Let also $\textstyle\boldsymbol{\Omega}_N = \Var(\frac{\sqrt{M}}{N}\sum_i\mathbf{m}_i^{\hat{P}}(\boldsymbol{\theta}_0))$. \\
We assume the following.
\begin{assumption}
$\boldsymbol{\Omega}_N = O_p(1)$ and $\plim \boldsymbol{\Omega}_N = \boldsymbol{\Omega}_0$
\end{assumption}
\noindent This assumption notably holds when the first stage estimator is a m-estimator.

%Other $\boldsymbol{\theta}$ could not be root-$M$ consistent and normally distributed asymptotically. We set the assumption for the general when the first stage estimator is not an M-estimator. This assumption is  the main requirement of our approach to estimate the variance of $\boldsymbol{\theta}$.

Under this assumption, we have
$$\boldsymbol{\Sigma}_0 = \mathbf{H}_0 \boldsymbol{\Omega}_0 \mathbf{H}_0^{\prime}.$$
\noindent Let $\boldsymbol{\zeta}_{N,m}^{\hat{P}}$ be the sum of $\mathbf{m}_i^{\hat{P}}(\boldsymbol{\theta}_0)$ over the $m$-th sub-network and let $\boldsymbol{\zeta}_{N,m}^{P}$ be the same statistic where $\hat{P}$ is replaced by $P$. 
In practice, $\mathbf{H}_0$ can be estimated consistently by, $$\textstyle\hat{\mathbf{H}}_0 = N\left[\sum_i\dfrac{\partial\mathbf{m}_i^{\hat{P}}(\hat{\boldsymbol{\theta}})^{\prime}}{\partial\boldsymbol{\theta}} \mathbf{W}_N \sum_i\dfrac{\partial\mathbf{m}_i^{\hat{P}}({\hat{\boldsymbol{\theta}}})}{\partial\boldsymbol{\theta}^{\prime}}\right]^{-1}\sum_i\dfrac{\partial\mathbf{m}_i^{\hat{P}}(\hat{\boldsymbol{\theta}})^{\prime}}{\partial\boldsymbol{\theta}} \mathbf{W}_N.$$
\noindent On the other hand, $\boldsymbol{\Sigma}_0$ can be estimated by $\boldsymbol{\Sigma}_N$, where
\begin{align}
    \textstyle\boldsymbol{\Sigma}_N &=\textstyle \Exp(\Var(\frac{\sqrt{M}}{N}\sum_m\boldsymbol{\zeta}_{N,m}^{\hat{P}}|{\hat{P}})) + \Var(\Exp(\frac{\sqrt{M}}{N}\sum_m\boldsymbol{\zeta}_{N,m}^{\hat{P}}|{\hat{P}})), \nonumber\\
    \textstyle\boldsymbol{\Sigma}_N &=\textstyle \frac{M}{N^2}\Exp(\sum_m\Var(\boldsymbol{\zeta}_{N,m}^{\hat{P}}|{\hat{P}})) + \frac{M}{N^2}\Var(\sum_m\Exp(\boldsymbol{\zeta}_{N,m}^{\hat{P}}|{\hat{P}})). \nonumber
\end{align}
The term $\textstyle N^{-1}\Exp(\sum_m\Var(\boldsymbol{\zeta}_{N,m}^{\hat{P}}|{\hat{P}}))$ is due to the error term of the model $\boldsymbol{\varepsilon}$ and the fact that the true network is not observed whereas $\textstyle N^{-1}\Var(\sum_m\Exp(\boldsymbol{\zeta}_{N,m}^{\hat{P}}|{\hat{P}}))$ is due to uncertainty associated with the estimation of $P$.
In practice, we can compute an estimator of $\textstyle \boldsymbol{\zeta}_{N,m}^{\hat{P}}$, $m = 1, ..., M$ by replacing $\boldsymbol{\theta}_0$ by its consistent estimator $\hat{\boldsymbol{\theta}}$. Thus, we can also estimate $\textstyle \sum_m\Var(\boldsymbol{\zeta}_{N,m}^{\hat{P}}|{\hat{P}})$ and $\textstyle \sum_m\Exp(\boldsymbol{\zeta}_{N,m}^{\hat{P}}|{\hat{P}})$. With several simulations from the distribution of $\hat{P}$, we finally compute $\boldsymbol{\Sigma}_N$.\footnote{Our R package offers tools to compute this variance. See also our online appendix.}

\cleardoublepage

\begin{center}
    \LARGE Online Appendix
\end{center}

\section{Additional Results}\label{sec:appendix_otherresults}

\subsection{Simple estimators}

\begin{proposition}\label{prop:all_observed}
[Conditions] Suppose that $\mathbf{GX}$ and $\mathbf{Gy}$ are observed. Let $\boldsymbol{H}$ be a matrix such that: (1) at least one column of $\mathbf{H}^k\mathbf{X}$ is (strongly) correlated with $\mathbf{G}\mathbf{y}$, conditional on $[\mathbf{1},\mathbf{X},\mathbf{GX}]$ for $k\geq 2$, and (2) $\mathbb{E}[\boldsymbol{\varepsilon}|\mathbf{X},\mathbf{H}]=\mathbf{0}$. Finally,  define the matrix $\mathbf{Z}=[\mathbf{1},\mathbf{X},\mathbf{GX},\mathbf{H}^2\mathbf{X},\mathbf{H}^3\mathbf{X}...]$.

[Results] Then, under classical assumptions (e.g. \cite{cameron2005microeconometrics}, Proposition 6.1), the (linear) GMM estimator based on the moment function $\frac{1}{N}\sum_i\mathbf{Z}_k'\boldsymbol{\varepsilon}_i$ is consistent and asymptotically normally distributed with the usual asymptotic variance-covariance matrix.
\end{proposition}

Condition (1) is the relevancy condition, while condition (2) is the exogeneity condition.\footnote{While (for simplicity) in Proposition \ref{prop:all_observed}, we use the entire matrix $\mathbf{X}$ in order to generate the instruments $\mathbf{HX}$, in practice, one should avoid including instruments (i.e. columns of $\mathbf{HX}$) that are weakly correlated with $\mathbf{Gy}$.} While Proposition \ref{prop:all_observed} holds for any matrix $\mathbf{H}$ such that conditions (1) and (2), the most sensible example in our context is when $\mathbf{H}$ is constructed using a draw from $\hat{P}(\mathbf{G})$.

Importantly, the moment conditions remain valid even when the researcher uses a \emph{mispecified} estimator of the distribution ${P}(\mathbf{G})$, as long as the specification error on $P(\mathbf{G})$ does not induce a correlation with $\boldsymbol{\varepsilon}$.\footnote{We would like to thank Chih-Sheng Hsieh and Arthur Lewbel for discussions on this important point.} This could be of great practical importance, especially if the estimation of $\hat{P}(\mathbf{G})$ suffers from small sample bias.% We provide an example in Section \ref{sec:ard} below.

We present a simple, asymptotically biased, linear GMM estimator. The presentation of such this estimator is useful for two reasons. First, simulations show that the asymptotic bias turns out to be negligible in many cases, especially for moderate group sizes. Moreover, the estimator is computationally attractive since the estimator can be written in closed-form. Second, the estimator helps to understand the logic underlying the estimator defined in Theorem \ref{prop:non_observed}, which we can view as a bias-corrected version of this simple linear GMM estimator. Proposition \ref{prop:bias_nocontext} formalizes.

\begin{proposition}\label{prop:bias_nocontext}
[Conditions] Assume that $\mathbf{GX}$ is observed. Let $\ddot{\mathbf{S}}=[\mathbf{1},\mathbf{X},\mathbf{GX},\ddot{\mathbf{G}}\mathbf{X},\ddot{\mathbf{G}}\mathbf{y}]$ and $\dot{\mathbf{Z}}=[\mathbf{1},\mathbf{X},\mathbf{GX},\ddot{\mathbf{G}}\mathbf{X},\dot{\mathbf{G}}^2\mathbf{X},\dot{\mathbf{G}}^3\mathbf{X},...]$. Denote by $\hat{\boldsymbol{\theta}}$ the linear GMM estimator based on the (pseudo) moment function $\frac{1}{N}\sum_i \dot{\mathbf{Z}}_i[\boldsymbol{\eta}_i+\boldsymbol{\varepsilon}_i]$, and define the sensitivity matrix\newline ${\mathbf{M}}_N=[(\ddot{\mathbf{S}}'\dot{\mathbf{Z}}/N)\mathbf{W}(\dot{\mathbf{Z}}'\ddot{\mathbf{S}}/N)]^{-1}(\ddot{\mathbf{S}}'\dot{\mathbf{Z}}/N)\mathbf{W}$.

[Result] Then, under classical assumptions (see proof), the asymptotic bias of $\hat{\boldsymbol{\theta}}$ is given by $\alpha \mathbf{M}_0 \plim[\dot{\mathbf{Z}}'({\mathbf{G}}-\ddot{\mathbf{G}})\mathbf{y}/N]$. Moreover, letting $\mathbf{W}=\mathbf{I}$ minimizes the asymptotic bias in the sense of minimizing the Frobenius norm of $\mathbf{M}$.
\end{proposition}
While there are no obvious way to get a consistent estimate of the asymptotic bias (because $\mathbf{y}$ is a function of $\mathbf{G}$) simulations show that the bias is very small in practice.\footnote{See Section \ref{sec:ard} below.} 

The intuition behind Proposition \ref{prop:bias_nocontext} comes from the literature on error-in-variable models with repeated observations (e.g. \cite{bound2001measurement}). The instrumental variable uses two independent draws from the (estimated) distribution of the true network. One draw is used to proxy the unobserved variable (i.e. $\mathbf{Gy}$), while the other is used to proxy the instrument (i.e. $\mathbf{G}\mathbf{X}$). This approach greatly reduces the bias as compared to a situation in which only one draw would be used.\footnote{Simulations available uppon request.}

The argument in Proposition \ref{prop:bias_nocontext} is very similar to the one in \cite{andrews2017measuring}, although here perturbation with respect to the true model is not \textit{local}.\footnote{See page 1562 in \cite{andrews2017measuring}.} We also show that we expect $\mathbf{W}=\mathbf{I}$ to minimize the asymptotic bias. Our result therefore provides a theoretical justification for the simulations in \cite{onishi2021sample} who show that the using the identity matrix to weight the moments greatly reduce the bias in the context studied by \cite{andrews2017measuring}.

\subsubsection{Proof of Proposition \ref{prop:bias_nocontext}}
\noindent\textbf{Part 1: Asymptotic bias}
Define $\boldsymbol{\Delta}=\mathbf{G}-\ddot{\mathbf{G}}$ and rewrite $\boldsymbol{\eta}=\alpha[\mathbf{G}-\ddot{\mathbf{G}}]\mathbf{y}=\alpha\boldsymbol{\Delta}\mathbf{y}$. Let $\boldsymbol{\theta}_0^+ = (\boldsymbol{\theta}_0^{\prime}, 0, 0, \dots, 0)^{\prime}$ be the true value the parameter when regressors are defined as: $\ddot{\mathbf{S}}=[\mathbf{1},\mathbf{X},\mathbf{GX},\ddot{\mathbf{G}}\mathbf{X},\ddot{\mathbf{G}}\mathbf{y}]$.
The Linear GMM estimator can be written as:
\begin{align*}
    &\textstyle\hat{\boldsymbol{\theta}}=\left[\left(\frac{\ddot{\mathbf{S}}'\dot{\mathbf{Z}}}{N}\right)\left(\frac{\dot{\mathbf{Z}}'\ddot{\mathbf{S}}}{N}\right)\right]^{-1}\left(\frac{\ddot{\mathbf{S}}'\dot{\mathbf{Z}}}{N}\right)\left(\frac{\dot{\mathbf{Z}}'\ddot{\mathbf{S}}}{N}\boldsymbol{\theta}_0^+ + \frac{ \dot{\mathbf{Z}}'[\boldsymbol{\eta}+\boldsymbol{\varepsilon}]}{N}\right),\\
    &\textstyle\hat{\boldsymbol{\theta}}=\boldsymbol{\theta}_0^+ + \mathbf{M}_N\left(\frac{ \dot{\mathbf{Z}}'\boldsymbol{\eta}+\dot{\mathbf{Z}}'\boldsymbol{\varepsilon}}{N}\right),
\end{align*}
where $\textstyle\mathbf{M}_N = \left[\left(\frac{\ddot{\mathbf{S}}'\dot{\mathbf{Z}}}{N}\right)\left(\frac{\dot{\mathbf{Z}}'\ddot{\mathbf{S}}}{N}\right)\right]^{-1}\left(\frac{\ddot{\mathbf{S}}'\dot{\mathbf{Z}}}{N}\right)$.\\
\noindent The asymptotic bias of $\hat{\boldsymbol{\theta}}$ is then given by $\textstyle \plim \boldsymbol{\theta}_N^{\ast} = \alpha \mathbf{M}_0 \plim[\dot{\mathbf{Z}}'({\mathbf{G}}-\ddot{\mathbf{G}})\mathbf{y}/N]$.

\noindent\textbf{Part 2: Choice of $\mathbf{W}$}
Let $\mathbf{K}=\dot{\mathbf{Z}}'\boldsymbol{\Delta}\mathbf{G}^2/N$ if $\boldsymbol{\gamma}=\mathbf{0}$ and $\mathbf{K}=\dot{\mathbf{Z}}'\boldsymbol{\Delta}/N$ otherwise. Consider $\Vert \mathbf{MK}\Vert_F=\sqrt{trace(\mathbf{K}'\mathbf{M}'\mathbf{M}\mathbf{K})}=\sqrt{trace(\mathbf{K}\mathbf{K}'\mathbf{M}'\mathbf{M})}$. We have:
$$
(1/N^2)\mathbf{M}\mathbf{M}'=[\ddot{\mathbf{S}}'\dot{\mathbf{Z}}\mathbf{W}\dot{\mathbf{Z}}'\ddot{\mathbf{S}}]^{-1}\ddot{\mathbf{S}}'\dot{\mathbf{Z}}\mathbf{W}\mathbf{W}\dot{\mathbf{Z}}'\ddot{\mathbf{S}}[\ddot{\mathbf{S}}'\dot{\mathbf{Z}}\mathbf{W}\dot{\mathbf{Z}}'\ddot{\mathbf{S}}]^{-1}
$$
Let $\mathbf{W}=\mathbf{C}'\mathbf{C}$ and let $\mathbf{B}=\ddot{\mathbf{S}}'\dot{\mathbf{Z}}\mathbf{C}'$. We have:
$$
(1/N^2)\mathbf{M}\mathbf{M}'=(\mathbf{B}'\mathbf{B})^{-1}\mathbf{B}'\mathbf{C}\mathbf{C}'
\mathbf{B}(\mathbf{B}'\mathbf{B})^{-1}
$$
Now, define $\mathbf{J}'=(\mathbf{B}'\mathbf{B})^{-1}\mathbf{B}'\mathbf{C}-(\mathbf{B}'(\mathbf{C}')^{-1}\mathbf{C}^{-1}\mathbf{B})^{-1}\mathbf{B}'(\mathbf{C}')^{-1}$. We have:
$$
(1/N^2)\mathbf{M}\mathbf{M}'=\mathbf{J}'\mathbf{J}+(\mathbf{B}'(\mathbf{C}')^{-1}\mathbf{C}^{-1}\mathbf{B})^{-1}=\mathbf{J}'\mathbf{J}+ (\ddot{\mathbf{S}}'\dot{\mathbf{Z}}\dot{\mathbf{Z}}'\ddot{\mathbf{S}})^{-1}
$$
Therefore, we have:
$$
(1/N^2)\Vert \mathbf{M}\Vert_F=\sqrt{trace(\mathbf{J}'\mathbf{J}+ (\ddot{\mathbf{S}}'\dot{\mathbf{Z}}\dot{\mathbf{Z}}'\ddot{\mathbf{S}})^{-1})}=\sqrt{trace(\mathbf{J}'\mathbf{J})+ trace((\ddot{\mathbf{S}}'\dot{\mathbf{Z}}\dot{\mathbf{Z}}'\ddot{\mathbf{S}})^{-1})}
$$
When $\mathbf{W}=\mathbf{I}$, we have that $\mathbf{J}=\mathbf{0}$ and the Frobenius norm of $\mathbf{M}$ is given by $N^2\sqrt{trace((\ddot{\mathbf{S}}'\dot{\mathbf{Z}}\dot{\mathbf{Z}}'\ddot{\mathbf{S}})^{-1})}$.

\subsubsection{Bias correction for $\mathbf{GX}$ observed}

Let us replace $\ddot{\mathbf{V}}$ with $\mathbf{V}$ in (\ref{eq:bias_corr}). We have:
$$
\dot{\mathbf{Z}}^{(r)\prime}_i\left[(\mathbf{I}-\alpha\dddot{\mathbf{G}}^{(t)})_i\left((\mathbf{I}-\alpha{\mathbf{G}})^{-1}-(\mathbf{I}-\alpha\ddot{\mathbf{G}}^{(s)})^{-1}\right)\mathbf{V}\tilde{\boldsymbol{\theta}}\right]
$$
which is equal to:
$$
\dot{\mathbf{Z}}^{(r)\prime}_i\left[(\mathbf{I}-\alpha\dddot{\mathbf{G}}^{(t)})_i\left((\mathbf{I}-\alpha{\mathbf{G}})^{-1}-(\mathbf{I}-\alpha\ddot{\mathbf{G}}^{(s)})^{-1}\right)\left((\mathbf{I}-\alpha\mathbf{G})\mathbf{y} + \boldsymbol{\varepsilon}\right)\right]
%\mathbb{E}\dot{\mathbf{Z}}(\mathbf{I}-\alpha\dddot{\mathbf{G}})(\mathbf{I}-\alpha\ddot{\mathbf{G}})^{-1}(\mathbf{I}-\alpha\ddot{\mathbf{G}})[(\mathbf{I}-\alpha{\mathbf{G}})^{-1}-(\mathbf{I}-\alpha\ddot{\mathbf{G}})^{-1}](\mathbf{I}-\alpha{\mathbf{G}})(\mathbf{I}-\alpha{\mathbf{G}})^{-1}\mathbf{V}\tilde{\boldsymbol{\theta}}
$$
which simplifies to:
$$
\dot{\mathbf{Z}}^{(r)\prime}_i(\mathbf{I}-\alpha\dddot{\mathbf{G}}^{(t)})_i(\mathbf{I}-\alpha\ddot{\mathbf{G}}^{(s)})^{-1}[\alpha({\mathbf{G}}-\ddot{\mathbf{G}}^{(s)})]\mathbf{y} + \dot{\mathbf{Z}}^{(r)\prime}_i\left[(\mathbf{I}-\alpha\dddot{\mathbf{G}}^{(t)})_i\left((\mathbf{I}-\alpha{\mathbf{G}})^{-1}-(\mathbf{I}-\alpha\ddot{\mathbf{G}}^{(s)})^{-1}\right)\boldsymbol{\varepsilon}\right]
$$
\noindent Note that the expectation of the term $\dot{\mathbf{Z}}^{(r)\prime}_i\left[(\mathbf{I}-\alpha\dddot{\mathbf{G}}^{(t)})_i\left((\mathbf{I}-\alpha{\mathbf{G}})^{-1}-(\mathbf{I}-\alpha\ddot{\mathbf{G}}^{(s)})^{-1}\right)\boldsymbol{\varepsilon}\right]$  is null.

\subsubsection{Corollaries}
\begin{corollary}\label{prop:GXobs}
Assume that $\mathbf{GX}$ is observed, but that $\mathbf{Gy}$ is not observed. Let $\dot{\mathbf{Z}}^{(s)}=[\mathbf{1},\mathbf{X},{\mathbf{G}}\mathbf{X},\dot{\mathbf{G}}^{s}{\mathbf{G}}\mathbf{X},(\dot{\mathbf{G}}^{(s)})^2{\mathbf{G}}\mathbf{X},...]$,
$\ddot{\mathbf{Z}}^{(s,t)}=[\mathbf{1},\mathbf{X},\ddot{\mathbf{G}}^{(t)}\mathbf{X},\dot{\mathbf{G}}^{s}\ddot{\mathbf{G}}^{(t)}\mathbf{X},(\dot{\mathbf{G}}^{(s)})^2\ddot{\mathbf{G}}^{(t)}\mathbf{X},...]$, $\mathbf{V}=[\mathbf{1},\mathbf{X},\mathbf{G}\mathbf{X}]$, and $\ddot{\mathbf{V}}^{(t)}=[\mathbf{1},\mathbf{X},\ddot{\mathbf{G}}^{(t)}\mathbf{X}]$. Then, the results from Theorem \ref{prop:non_observed} hold for the following (simulated) moment function:
\begin{eqnarray}\label{eq:Gyobs}
\frac{1}{S}\sum_{s=1}^S\dot{\mathbf{Z}}_i^{(s)\prime}(\mathbf{I}-\alpha\dot{\mathbf{G}}^{(s)})_i\mathbf{y} -
\frac{1}{ST}\sum_{t=1}^T\sum_{s=1}^S (\dot{\mathbf{Z}}^{(s)\prime}\mathbf{V}-\ddot{\mathbf{Z}}^{(s,t)\prime}\ddot{\mathbf{V}}^{(t)})_i\tilde{\boldsymbol{\theta}}\nonumber\\ -\frac{1}{ST}\sum_{t=1}^T\sum_{s=1}^S  \ddot{\mathbf{Z}}^{(s,t)\prime}_i(\mathbf{I}-\alpha\dot{\mathbf{G}}^{(s)})_i(\mathbf{I}-\alpha\ddot{\mathbf{G}}^{(t)})^{-1}\ddot{\mathbf{V}}^{(t)}\tilde{\boldsymbol{\theta}}
\end{eqnarray}
\end{corollary}

\begin{corollary}\label{prop:Gyobs}
Assume that $\mathbf{Gy}$ is observed, but that $\mathbf{GX}$ is not observed. Let $\dot{\mathbf{Z}}^{(s)}=[\mathbf{1},\mathbf{X},\dot{\mathbf{G}}^{(s)}\mathbf{X},(\dot{\mathbf{G}}^{(s)})^2\mathbf{X},...]$, and $\ddot{\mathbf{V}}^{(t)}=[\mathbf{1},\mathbf{X},\ddot{\mathbf{G}}^{(t)}\mathbf{X}]$.  Then, the results from Theorem \ref{prop:non_observed} hold for the following (simulated) moment function:
\begin{eqnarray}\label{eq:GXobs}
\frac{1}{S}\sum_{s=1}^S\dot{\mathbf{Z}}_i^{(s)\prime}(\mathbf{I}-\alpha\mathbf{G})_i\mathbf{y} -
\frac{1}{ST}\sum_{t=1}^T\sum_{s=1}^S \dot{\mathbf{Z}}^{(s)\prime}_i\ddot{\mathbf{V}}^{(t)}_i\tilde{\boldsymbol{\theta}}
\end{eqnarray}
\end{corollary}
