# Supplementary material for: Estimating Peer Effects Using Partial Network Data
Source: arXiv:2509.08145 source file (2025-09-09)
Supplement: Supplementary file 16 [file appendix_proof.tex]

\section{SGMM estimator}\label{sec:appendix_proofs}

Throughout, otherwise stated, the subscript zero is used to denote the true value of a parameter. 
Consider the following regularity assumptions.

\begin{assumption}\label{as:regularity}
$\boldsymbol{\rho}_0\in int(\mathcal{R})$ and $\boldsymbol{\theta}_0\in int(\Theta)$, where $\mathcal{R}$ and $\Theta$ are both compact subsets of the Euclidean space.
\end{assumption}

\begin{assumption}\label{as:nonsingular}
For all $r=1,...,R$, $s=1,...,S$, and $t=1,...,T$, $(\mathbf{I}-\alpha \dot{\mathbf{G}}^{r})$, $(\mathbf{I}-\alpha \ddot{\mathbf{G}}^{s})$ and $(\mathbf{I}-\alpha \dddot{\mathbf{G}}^{t})$ are non-singular
\end{assumption}
In particular, when $\mathbf{G}$ is row-normalized (so $\dot{\mathbf{G}}^{r}$, $\ddot{\mathbf{G}}^{s}$, and $\dddot{\mathbf{G}}^{t}$ are also row-normalized), Assumption \ref{as:alpha} implies Assumption \ref{as:nonsingular}. Assumption \ref{as:regularity:boundedsupp} below ensures that the moment function is uniformly bounded.

\begin{assumption}\label{as:regularity:boundedsupp}
$\mathbf{X}_i^{\prime}$ is uniformly bounded in $i$. The $(i,j)$-th entries of $\mathbf{G}$ (so $\dot{\mathbf{G}}^{r}$, $\ddot{\mathbf{G}}^{s}$, and $\dddot{\mathbf{G}}^{t}$) are  uniformly bounded in $i$ and $j$.
\end{assumption}

\bigskip
We consider an objective function for the GMM estimator of the usual form: $$\mathcal{Q}_N(\boldsymbol{\theta}) =  \textstyle\left(\frac{1}{N}\sum_i \mathbf{m}_i(\boldsymbol{\theta})\right)'\mathbf{W}_N\left(\frac{1}{N}\sum_i \mathbf{m}_i(\boldsymbol{\theta})\right),$$
where $\mathbf{m}_i(\boldsymbol{\theta})$ is the moment function and $\mathbf{W}_N$ is positive definite.

\begin{assumption}\label{as:weigth}
$\mathcal{Q}_N(\boldsymbol{\theta})$ converges in probability to some $\mathcal{Q}_0(\boldsymbol{\theta})$.
\end{assumption}

The identification condition is discussed in Section \ref{app:ident} (see in particular Assumptions \ref{as:convex} and \ref{as:globalmin}).
%\begin{assumption}\label{as:moment:null}
%$\textstyle\plim\mathbb{E}\textstyle\left(\frac{1}{N}\sum_i \mathbf{m}_i({\boldsymbol{\theta}})\right)=\mathbf{0}$ iff ${\boldsymbol{\theta}}={\boldsymbol{\theta}}_0$.
%\end{assumption}

\subsection{Proof of Theorem \ref{prop:non_observed}}

Let $$\textstyle\mathbf{m}_i(\boldsymbol{\theta})=\frac{1}{RST}\sum_r\sum_s\sum_t\dot{\mathbf{Z}}_i^{(r)\prime}(\mathbf{I}-\alpha\dddot{\mathbf{G}}^{(t)})_i\left(\mathbf{y}-(\mathbf{I}-\alpha\ddot{\mathbf{G}}^{(s)})^{-1}\ddot{\mathbf{V}}^{(s)}\tilde{\boldsymbol{\theta}}\right) .$$

We will show that, by construction, we have $\textstyle\plim\mathbb{E}\left(\mathbf{m}_i(\boldsymbol{\theta}_0)\right)=\mathbf{0}$ for any finite $S$ and $T$, where $\plim$ is the probability limit.

To see why, let us substitute $\mathbf{y}=(\mathbf{I}-\alpha_0\mathbf{G})^{-1}(\mathbf{V}\tilde{\boldsymbol{\theta}}_0+\boldsymbol{\varepsilon})$ in the moment function. We have
\begin{eqnarray*}
\textstyle\mathbf{m}_i(\boldsymbol{\theta}_0)&=&\textstyle\frac{1}{RST}\sum_r\sum_s\sum_t \dot{\mathbf{Z}}_i^{(r)\prime}(\mathbf{I}-\alpha_0\dddot{\mathbf{G}}^{(t)})_i\left[(\mathbf{I}-\alpha_0\mathbf{G})^{-1}\mathbf{V}-(\mathbf{I}-\alpha_0\ddot{\mathbf{G}}^{(s)})^{-1}\ddot{\mathbf{V}}^{(s)}\right]\tilde{\boldsymbol{\theta}}_0\\
&+&\textstyle\frac{1}{RS}\sum_r\sum_s \dot{\mathbf{Z}}_i^{(r)\prime}(\mathbf{I}-\alpha_0\dddot{\mathbf{G}}^{(t)})_i(\mathbf{I}-\alpha_0\mathbf{G})^{-1}\boldsymbol{\varepsilon} .
\end{eqnarray*}

Consider the second term first. For any $r,~s,~t$, we have
$$\textstyle
\mathbb{E}\left(\dot{\mathbf{Z}}_i^{(r)\prime}(\mathbf{I}-\alpha_0\dddot{\mathbf{G}}^{(t)})_i(\mathbf{I}-\alpha_0\mathbf{G})^{-1}\boldsymbol{\varepsilon}\right)=\mathbf{0},
$$
directly from Assumption \ref{as:exonet} and the specification of the network formation process (see Assumption \ref{as:partial}).

Consider now the first term. We need
$$\textstyle
\plim \mathbb{E}\left[\dot{\mathbf{Z}}_i^{(r)\prime}(\mathbf{I}-\alpha_0\dddot{\mathbf{G}}^{(t)})_i\left[(\mathbf{I}-\alpha_0\mathbf{G})^{-1}\mathbf{V}-(\mathbf{I}-\alpha_0\ddot{\mathbf{G}}^{(s)})^{-1}\ddot{\mathbf{V}}^{(s)}\right]\tilde{\boldsymbol{\theta}}_0\right]=\mathbf{0}.
$$

\noindent Note that, for N fixed, $\mathbf{G}$, $\dot{\mathbf{G}}^{(r)}$, $\ddot{\mathbf{G}}^{(s)}$, and $\dddot{\mathbf{G}}^{(t)}$ have a finite number of possible realizations. Thus, $\textstyle\mathbb{E}\left[\dot{\mathbf{Z}}_i^{(s)\prime}(\mathbf{I}-\alpha_0\dddot{\mathbf{G}}^{(t)})_i(\mathbf{I}-\alpha_0\mathbf{G})^{-1}\mathbf{V}\tilde{\boldsymbol{\theta}}_0\right]$ can be written as a continuous function of $P$, the distribution of the adjacency matrix, and $\hat{P}$, a consistent estimator of that distribution.\footnote{The function would essentially composed of summations and products of terms depending on $P$ and $\hat{P}$.} Analogously, $\mathbb{E}\left[\dot{\mathbf{Z}}_i^{(s)\prime}(\mathbf{I}-\alpha_0\dddot{\mathbf{G}}^{(t)})_i(\mathbf{I}-\alpha_0\ddot{\mathbf{G}}^{(s)})^{-1}\ddot{\mathbf{V}}^{(s)}\tilde{\boldsymbol{\theta}}_0\right]$ also can be written as a same function with the difference that $P$ is replaced by $\hat{P}$. As both functions are continuous and because $\hat{P}$ converges in probability to $P$ (see Assumption \ref{as:partial}), their limits are obtained by replacing $\hat{P}$ by $P$ and are therefore equal. As such, we have
$$
\plim \mathbb{E}\left[\dot{\mathbf{Z}}_i^{(s)\prime}(\mathbf{I}-\alpha_0\dddot{\mathbf{G}}^{(t)})_i(\mathbf{I}-\alpha_0\mathbf{G})^{-1}\mathbf{V}\tilde{\boldsymbol{\theta}}_0\right]=\plim \mathbb{E}\left[\dot{\mathbf{Z}}_i^{(s)\prime}(\mathbf{I}-\alpha_0\dddot{\mathbf{G}}^{(t)})_i(\mathbf{I}-\alpha_0\ddot{\mathbf{G}}^{(s)})^{-1}\ddot{\mathbf{V}}^{(s)}\tilde{\boldsymbol{\theta}}_0\right].
$$

\noindent The GMM estimator
$$\textstyle
\hat{\boldsymbol{\theta}}=\arg\max \mathcal{Q}_N(\boldsymbol{\theta})
$$
is therefore consistent under Assumptions \ref{as:alpha}--\ref{as:weigth} if no other $\boldsymbol{\theta}$ solves the moment condition (e.g. see \cite{newey1994large}; Theorem 2.6). The next section discusses the numerical implementation and identification of the estimator.

\subsubsection{Concentration and Identification\label{app:ident}}
Although the GMM estimator could be solved numerically, it is helpful to concentrate the objective function around $\alpha$.
Let $\textstyle\mathbf{R}(\alpha)=\frac{1}{RST}\sum_r\sum_s\sum_t\dot{\mathbf{Z}}^{(s)\prime}(\mathbf{I}-\alpha\dddot{\mathbf{G}}^{(t)})(\mathbf{I}-\alpha\ddot{\mathbf{G}}^{(s)})^{-1}\ddot{\mathbf{V}}^{(s)}/N$ and $\textstyle\mathbf{D}(\alpha)=\frac{1}{RST}\sum_r\sum_s\sum_t\dot{\mathbf{Z}}^{(s)\prime}(\mathbf{I}-\alpha\dddot{\mathbf{G}}^{(t)})/N$ so that $\textstyle\frac{1}{N}\sum_i\mathbf{m}_i(\boldsymbol{\theta})=\mathbf{D}(\alpha)\mathbf{y}-\mathbf{R}(\alpha)\tilde{\boldsymbol{\theta}}$.

The gradient of the objective function with respect to $\textstyle\tilde{\boldsymbol{\theta}}$ is
$$
\textstyle-2\left(\mathbf{D}(\alpha)\mathbf{y}-\mathbf{R}(\alpha)\tilde{\boldsymbol{\theta}}\right)'\mathbf{W}_N\mathbf{R(\alpha)}.
$$
The hessian is therefore $2\mathbf{R}'(\alpha)\mathbf{W}_N\mathbf{R(\alpha)}$, which is semi-positive definite. Hence, the following assumption ensures identification of $\tilde{\boldsymbol{\theta}}$, conditional on $\alpha$. %Let $\textstyle\tilde{\mathbf{R}}(\alpha)=\frac{1}{RST}\sum_r\sum_s\sum_t\dot{\mathbf{Z}}^{(s)\prime}(\mathbf{I}-\alpha\dddot{\mathbf{G}}^{(t)})(\mathbf{I}-\alpha_0\ddot{\mathbf{G}}^{(s)})^{-1}\mathbf{V}^{(s)}/N$.

\begin{assumption}\label{as:convex}
For all $\alpha$, (a) $\mathbf{R}(\alpha)$ is a full rank matrix;
(b) %$\plim \mathbf{R}(\alpha)$ and $\plim \tilde{\mathbf{R}}(\alpha)$ exist and are denoted by $\mathbf{R}_0(\alpha)$ and $\tilde{\mathbf{R}}_0(\alpha)$ respectively;  
$\plim \mathbf{R}(\alpha)^{\prime} \mathbf{W}_N \mathbf{R}(\alpha)$ exists and is nonsingular.
\end{assumption}
\noindent Condition (a) ensures that the estimator is uniquely defined: assuming that $\mathbf{R}(\alpha)$ is a full rank matrix implies that $\left(\mathbf{D}(\alpha)\mathbf{y}-\mathbf{R}(\alpha)\tilde{\boldsymbol{\theta}}\right)'\mathbf{W}_N\mathbf{R(\alpha)}=\mathbf{0}$ holds for a single value of $\tilde{\boldsymbol{\theta}}$. Condition (b) ensures the identification is conditional on $\alpha$.

%\noindent A sufficient condition is that $\mathbf{R}'(\alpha)$ has full rank, for all $\alpha$.\\
\noindent Under Assumption \ref{as:convex}, the estimator of $\tilde{\boldsymbol{\theta}}$ conditionally on $\alpha$ is\\ $\hat{\tilde{\boldsymbol{\theta}}}(\alpha)=(\mathbf{R}'(\alpha)\mathbf{W}_N\mathbf{R(\alpha)})^{-1}\mathbf{R}'(\alpha)\mathbf{W}_N\mathbf{D}(\alpha)\mathbf{y}$.\\
The objective function can then be concentrated around $\alpha$, as 
$$\textstyle
\mathcal{Q}^c_N(\alpha)=\left(\mathbf{D}(\alpha)\mathbf{y}-\mathbf{R}(\alpha)\hat{\tilde{\boldsymbol{\theta}}}(\alpha)\right)'\mathbf{W}_N\left(\mathbf{D}(\alpha)\mathbf{y}-\mathbf{R}(\alpha)\hat{\tilde{\boldsymbol{\theta}}}(\alpha)\right)/N^{2}.
$$
While we cannot easily ensure that this function is globally convex in $\alpha$, the behavior of the function is easy to study because $\alpha$ is unidimensional and has a bounded support (see Assumption \ref{as:alpha}). Note that numerically minimizing the concentrated objective function implicitly checks Assumption \ref{as:convex}. Our final assumption ensures the identification of $\alpha$.
\begin{assumption}\label{as:globalmin}
(a) $\mathcal{Q}^c_N(\alpha)$ is uniquely minimized, and (b) $\plim \mathcal{Q}^c_N(\alpha)$ is uniquely minimized at $\alpha_0$.
\end{assumption}
Again, condition (a) ensures that the estimator is well defined, whereas condition (b) is the identification condition.
%\noindent We have $\textstyle\frac{1}{N}\sum_i\mathbf{m}_i(\boldsymbol{\theta})=\tilde{\mathbf{R}}(\alpha)\tilde{\boldsymbol{\theta}}_0-\mathbf{R}(\alpha)\tilde{\boldsymbol{\theta}}+ \textstyle\mathbf{D}(\alpha)\boldsymbol{\varepsilon}$. Under Assumptions \ref{as:exonet}, \ref{as:regularity:boundedsupp}, and \ref{as:convex}, 
%$\plim (1/N)\sum_i\mathbf{m}_i(\boldsymbol{\theta})$ exists, so does $\plim \mathcal{Q}_N(\boldsymbol{\theta})$. In addition,  $\mathcal{Q}_N(\boldsymbol{\theta})$ is continuously derivable in $\boldsymbol{\theta}$ and the derivative is bounded by Assumption \ref{as:regularity:boundedsupp}. Therefore, equicontinuity follows and $\mathcal{Q}_N(\boldsymbol{\theta})$ uniformly converges to $\plim \mathcal{Q}_N(\boldsymbol{\theta})$ \cite[][Lemmas 2.8, 2.9]{newey1994large}. On the other hand, the stochastic dominance (by Assumption \ref{as:regularity:boundedsupp}) implies that $\textstyle\plim \mathcal{Q}_N(\boldsymbol{\theta}) = \left(\plim \mathbb{E}\left(\frac{1}{N}\sum_i \mathbf{m}_i(\boldsymbol{\theta})\right)\right)'\mathbf{W}_0\left(\plim \mathbb{E}\left(\frac{1}{N}\sum_i \mathbf{m}_i(\boldsymbol{\theta})\right)\right)$. Thus, $\plim \mathcal{Q}_N(\boldsymbol{\theta})$ is minimized at a unique point, i.e., $\boldsymbol{\theta}_0$. As a result $\hat{\boldsymbol{\theta}}$ converges to $\boldsymbol{\theta}_0$ as $N$ grows to infinity under Assumptions \ref{as:manymarkets}-\ref{as:globalmin} \cite[see][Theorem 2.1]{newey1994large}.

\subsection{Asymptotic Normality for Sequential M-Estimators}\label{sec:asymptnorm}
The challenge in showing the asymptotic normality of our estimator lies in our use of a sequential estimation strategy.

Here, we assume that the model can be written as a sequential m-estimator. If the first-stage estimator $\hat{\boldsymbol{\rho}}$ is an M-estimator, then it verifies the first-order conditions:
\begin{equation}\label{eq:dq1}
    \frac{1}{M}\sum_{m = 1}^M  \dfrac{\partial Q_{1,m}(\hat{\boldsymbol{\rho}})}{\partial  \boldsymbol{\rho}} = 0,
\end{equation} for some function $Q_{1,m}$. We assume that $Q_{1,m}(\boldsymbol{\rho})$ is twice continuously differentiable in $\boldsymbol{\rho}$. Note that even if the observational unit of the first stage is at the pair level, it is always possible to take the sum or the average of the moment condition at the pair level to produce a moment condition at the group level as in (\ref{eq:dq1}).

Consider now the second stage, i.e. our SGMM estimator. It can be written as an m-estimator, continuously differentiable in $\boldsymbol{\rho}$ (in a neighborhood of  $\boldsymbol{\rho}_0$), and twice continuously differentiable in $\boldsymbol{\theta}$:
\begin{equation}
    \label{eq:dq2}\frac{1}{M}\sum_{m=1}^M  \dfrac{\partial Q_{2,m}(\hat{\boldsymbol{\theta}}, \hat{\boldsymbol{\rho}})}{\partial  \boldsymbol{\theta}} = 0,
\end{equation}

where $Q_{2,m}(\boldsymbol{\theta}, \hat{\boldsymbol{\rho}}) = \mathcal{Q}_N(\boldsymbol{\theta})$ for all $\boldsymbol{\theta}$.

Note that here, $Q_{2,m}(\boldsymbol{\theta}, {\boldsymbol{\rho}})$ is not everywhere continuous in $\boldsymbol{\rho}$. Indeed, remark that we can rewrite $\dot{\mathbf{G}}=f(\{\dot{a}_{ij}\}_{ij})=f(\{\mathbbm{1}[P_{ij}(1|\hat{\boldsymbol{\rho}})\geq \dot{u}_{ij}]\}_{ij})$, where $\dot{u}_{ij}\sim_{iid}U[0,1]$, and similarly for $\ddot{\mathbf{G}}$ and $\dddot{\mathbf{G}}$. This is only a variable change and does not introduce any additional assumptions; however, it shows that, using a finite number of network draws, the moment function is not everywhere continuous in $\boldsymbol{\rho}$ because of the indicator function.

This is similar to the estimator proposed, for example, by \cite{mcfadden1989method}. Conditions for the asymptotic normality of non-smooth m-estimators can be found, for example, in Theorem 7.1 of \cite{newey1994large} and Section 3.2 of \cite{andrews1994empirical}.

\subsection{Variance Estimation}\label{sec:varestim}
Let  where $\boldsymbol{\Sigma}_0 = \plim \boldsymbol{\Sigma}_N$ and $\boldsymbol{\Sigma}_N = \Var(\sqrt{M}\hat{\boldsymbol{\theta}})$. We now present a simple approach to estimate $\boldsymbol{\Sigma}_0$. Our approach does not rely on the asymptotic normality and takes into account the uncertainty related to the estimation at the first stage.

\noindent  Taking the first derivative of the objective function at the second stage (for finite $R$,$S$,$T$ and conditional on $\hat{\mathbf{\rho}}$) with respect to $\boldsymbol{\theta}$, we have
$$
\dfrac{1}{N}\sum_i\frac{\partial\mathbf{m}_i^{\hat{P}}(\boldsymbol{\theta})^{\prime}}{\partial\boldsymbol{\theta}}\mathbf{W}_N\dfrac{1}{N}\sum_i\mathbf{m}_i^{\hat{P}}(\boldsymbol{\theta})=\mathbf{0}.
$$
By applying the mean value theorem to $\frac{1}{N}\sum_i\mathbf{m}_i^{\hat{P}}(\boldsymbol{\theta})$, we have
$$\textstyle\sqrt{M}(\hat{\boldsymbol{\theta}}-\boldsymbol{\theta}_0)=-\left[\dfrac{1}{N}\sum_i\frac{\partial\mathbf{m}_i^{\hat{P}}(\hat{\boldsymbol{\theta}})^{\prime}}{\partial\boldsymbol{\theta}} \mathbf{W}_N \frac{1}{N}\sum_i\frac{\partial\mathbf{m}_i^{\hat{P}}({\boldsymbol{\theta}^*})}{\partial\boldsymbol{\theta}^{\prime}}\right]^{-1}\frac{1}{N}\sum_i\frac{\partial\mathbf{m}_i^{\hat{P}}(\hat{\boldsymbol{\theta}})^{\prime}}{\partial\boldsymbol{\theta}} \mathbf{W}_N\frac{\sqrt{M}}{N}\sum_i\mathbf{m}_i^{\hat{P}}(\boldsymbol{\theta}_0),   $$
where $\boldsymbol{\theta}^*$ is some point between $\hat{\boldsymbol{\theta}}$ and $\boldsymbol{\theta}_0$.  \\
Let $\textstyle\mathbf{H}_N = \left[\dfrac{1}{N}\sum_i\frac{\partial\mathbf{m}_i^{\hat{P}}(\hat{\boldsymbol{\theta}})^{\prime}}{\partial\boldsymbol{\theta}} \mathbf{W}_N \frac{1}{N}\sum_i\frac{\partial\mathbf{m}_i^{\hat{P}}({\boldsymbol{\theta}^*})}{\partial\boldsymbol{\theta}^{\prime}}\right]^{-1}\frac{1}{N}\sum_i\frac{\partial\mathbf{m}_i^{\hat{P}}(\hat{\boldsymbol{\theta}})^{\prime}}{\partial\boldsymbol{\theta}} \mathbf{W}_N$ and let $\mathbf{H}_0 = \plim \mathbf{H}_N$.\\
We have $$\textstyle\sqrt{M}(\hat{\boldsymbol{\theta}}-\boldsymbol{\theta}_0)=-\mathbf{H}_N\frac{\sqrt{M}}{N}\sum_i\mathbf{m}_i^{\hat{P}}(\boldsymbol{\theta}_0).$$
Let also $\textstyle\boldsymbol{\Omega}_N = \Var(\frac{\sqrt{M}}{N}\sum_i\mathbf{m}_i^{\hat{P}}(\boldsymbol{\theta}_0))$. \\
We assume the following:
\begin{assumption}
$\plim \boldsymbol{\Omega}_N = \boldsymbol{\Omega}_0$ and $\plim \mathbf{H}_N = \mathbf{H}_0$ exist and are finite matrices.
\end{assumption}
%\noindent This assumption notably holds when the first stage estimator is a m-estimator and the smoother simulator is used to draws networks.

%Other $\boldsymbol{\theta}$ could not be root-$M$ consistent and normally distributed asymptotically. We set the assumption for the general when the first stage estimator is not an M-estimator. This assumption is  the main requirement of our approach to estimate the variance of $\boldsymbol{\theta}$.

Under this assumption, we have
$$\boldsymbol{\Sigma}_0 = \mathbf{H}_0 \boldsymbol{\Omega}_0 \mathbf{H}_0^{\prime}.$$
\noindent Let $\boldsymbol{\zeta}_{N,m}^{\hat{P}}$ be the sum of $\mathbf{m}_i^{\hat{P}}(\boldsymbol{\theta}_0)$ over the $m$-th sub-network and let $\boldsymbol{\zeta}_{N,m}^{P}$ be the same statistic where $\hat{P}$ is replaced by $P$. 
In practice, $\mathbf{H}_0$ can be estimated consistently by $$\textstyle\hat{\mathbf{H}}_0 = N\left[\sum_i\dfrac{\partial\mathbf{m}_i^{\hat{P}}(\hat{\boldsymbol{\theta}})^{\prime}}{\partial\boldsymbol{\theta}} \mathbf{W}_N \sum_i\dfrac{\partial\mathbf{m}_i^{\hat{P}}({\hat{\boldsymbol{\theta}}})}{\partial\boldsymbol{\theta}^{\prime}}\right]^{-1}\sum_i\dfrac{\partial\mathbf{m}_i^{\hat{P}}(\hat{\boldsymbol{\theta}})^{\prime}}{\partial\boldsymbol{\theta}} \mathbf{W}_N.$$
\noindent On the other hand, $\boldsymbol{\Sigma}_0$ can be estimated by $\boldsymbol{\Sigma}_N$, where
\begin{align}
    \textstyle\boldsymbol{\Sigma}_N &=\textstyle \Exp(\Var(\frac{\sqrt{M}}{N}\sum_m\boldsymbol{\zeta}_{N,m}^{\hat{P}}|{\hat{P}})) + \Var(\Exp(\frac{\sqrt{M}}{N}\sum_m\boldsymbol{\zeta}_{N,m}^{\hat{P}}|{\hat{P}})), \nonumber\\
    \textstyle\boldsymbol{\Sigma}_N &=\textstyle \frac{M}{N^2}\Exp(\sum_m\Var(\boldsymbol{\zeta}_{N,m}^{\hat{P}}|{\hat{P}})) + \frac{M}{N^2}\Var(\sum_m\Exp(\boldsymbol{\zeta}_{N,m}^{\hat{P}}|{\hat{P}})). \nonumber
\end{align}
The term $\textstyle N^{-1}\Exp(\sum_m\Var(\boldsymbol{\zeta}_{N,m}^{\hat{P}}|{\hat{P}}))$ is due to the error term of the model $\boldsymbol{\varepsilon}$ and the true network not being observed, whereas $\textstyle N^{-1}\Var(\sum_m\Exp(\boldsymbol{\zeta}_{N,m}^{\hat{P}}|{\hat{P}}))$ is due to uncertainty associated with the estimation of $P$.
In practice, we can compute an estimator of $\textstyle \boldsymbol{\zeta}_{N,m}^{\hat{P}}$, $m = 1, ..., M$ by replacing $\boldsymbol{\theta}_0$ by its consistent estimator $\hat{\boldsymbol{\theta}}$. Thus, we can also estimate $\textstyle \sum_m\Var(\boldsymbol{\zeta}_{N,m}^{\hat{P}}|{\hat{P}})$ and $\textstyle \sum_m\Exp(\boldsymbol{\zeta}_{N,m}^{\hat{P}}|{\hat{P}})$. With several simulations from the distribution of $\hat{P}$, we finally compute $\boldsymbol{\Sigma}_N$.\footnote{Our R package offers tools to compute this variance. See also our Online Appendix.}
