# Supplementary material for: Estimating Peer Effects Using Partial Network Data
Source: arXiv:2509.08145 source file (2025-09-09)
Supplement: Supplementary file 20 [file appendix_addhealth.tex]

%\begin{figure}[!h]
%    \centering
%    \caption{Simulations from the posterior distribution of the outcome model's parameters}
%    \label{fig:simutheta}
%    \includegraphics[scale = 0.37]{graphs/simutheta.pdf}
%\end{figure}

%\begin{figure}
%    \centering
%    \caption{Posterior density of the outcome model's parameters}
%    \label{fig:post}
%    \includegraphics[scale = 0.37]{graphs/denstheta.pdf}
%\end{figure}

%\begin{figure}
%    \centering
%    \caption{Simulations from the posterior distribution of the network formation model's parameters}
%    \label{fig:simurho}
%    \includegraphics[scale = 0.47]{graphs/simurho.pdf}
%\end{figure}

\begin{table}[h]
\small
\centering
\caption{Posterior distribution by controlling for either censoring or missing links} 
\label{tab:appendapplication} 
    \begin{adjustbox}{max width=0.8\textwidth}
\begin{tabular}{lld{5}d{3}d{3}d{5}d{3}d{3}}
\\[-1.8ex]
\toprule
      &       & \multicolumn{3}{c}{Censoring} & \multicolumn{3}{c}{Missing links} \\
\multicolumn{2}{l}{Statistic} & \multicolumn{1}{c}{Mean}  & \multicolumn{1}{c}{Std. Dev.} & \multicolumn{1}{c}{\textit{t}-stat} & \multicolumn{1}{c}{Mean}  & \multicolumn{1}{c}{Std. Dev.} & \multicolumn{1}{c}{\textit{t}-stat} \\
\midrule
                          & \multicolumn{7}{c}{\textbf{Peer effect model}}  \\ 
\multicolumn{2}{l}{Peer effects}                       & 0.351***    & (0.024)   & 14.718   & 0.565***     & (0.041)     & 13.844    \\
\multicolumn{2}{l}{\textbf{Own effects}}               &             &            &           &               &              &            \\
\multicolumn{2}{l}{Female}                      & 0.144***   & (0.029)   & 5.008   & 0.125***    & (0.031)     & 4.050    \\
\multicolumn{2}{l}{Hispanic}                    & -0.083**     & (0.042)   & -1.967    & -0.142**      & (0.047)     & -3.046     \\
\multicolumn{2}{l}{Race (White)}                &             &           &          &              &             &           \\
                          & Black               & -0.232***    & (0.046)   & -5.035    & -0.210***     & (0.056)     & -3.778     \\
                          & Asian               & -0.090       & (0.090)   & -0.999    & -0.119        & (0.091)     & -1.308     \\
                          & Other               & 0.053      & (0.051)   & 1.042   & 0.038       & (0.052)     & 0.721    \\
\multicolumn{2}{l}{Mother's education. (High)}            &             &           &          &              &             &           \\
                          & \textless High      & -0.123**     & (0.039)   & -3.182    & -0.123**      & (0.040)     & -3.102     \\
                          & \textgreater High   & 0.140***   & (0.034)   & 4.103   & 0.110**     & (0.034)     & 3.216    \\
                          & Missing             & -0.061       & (0.052)   & -1.172    & -0.064        & (0.051)     & -1.235     \\
\multicolumn{2}{l}{Mother's job (Stay-at-home)}         &             &           &          &              &             &           \\
                          & Professional        & 0.083*     & (0.044)   & 1.872   & 0.074*      & (0.044)     & 1.686    \\
                          & Other               & 0.004      & (0.035)   & 0.112   & -0.007        & (0.035)     & -0.199     \\
                          & Missing             & -0.065       & (0.047)   & -1.365    & -0.069        & (0.047)     & -1.450     \\
\multicolumn{2}{l}{age}                         & -0.074***    & (0.010)   & -7.745    & -0.079***     & (0.011)     & -7.317     \\
\multicolumn{2}{l}{\textbf{Contextual effects}}          &             &            &           &               &              &            \\
\multicolumn{2}{l}{Female}                      & 0.009      & (0.049)   & 0.177   & 0.053       & (0.094)     & 0.569    \\
\multicolumn{2}{l}{Hispanic}                    & 0.062      & (0.068)   & 0.905   & 0.356**     & (0.114)     & 3.117    \\
\multicolumn{2}{l}{Race (White)}                &             &           &          &              &             &           \\
                          & Black               & 0.053      & (0.059)   & 0.898   & 0.057       & (0.075)     & 0.754    \\
                          & Asian               & 0.233      & (0.184)   & 1.264   & 0.505       & (0.552)     & 0.916    \\
                          & Other               & -0.138       & (0.089)   & -1.538    & -0.240        & (0.182)     & -1.317     \\
\multicolumn{2}{l}{Mother's education (High)}            &             &           &          &              &             &           \\
                          & \textless High      & -0.271***    & (0.071)   & -3.833    & -0.373**      & (0.157)     & -2.383     \\
                          & \textgreater High   & 0.069      & (0.060)   & 1.154   & 0.067       & (0.111)     & 0.606    \\
                          & Missing             & -0.078       & (0.094)   & -0.833    & -0.024        & (0.191)     & -0.127     \\
\multicolumn{2}{l}{Mother's job (Stay-at-home)}         &             &           &          &              &             &           \\
                          & Professional        & -0.117       & (0.080)   & -1.474    & 0.024       & (0.150)     & 0.157    \\
                          & Other               & -0.107*      & (0.060)   & -1.767    & -0.038        & (0.112)     & -0.345     \\
                          & Missing             & -0.103       & (0.087)   & -1.190    & 0.004       & (0.184)     & 0.024    \\
\multicolumn{2}{l}{Age}                         & 0.067***   & (0.006)   & 11.441  & 0.091***    & (0.009)     & 9.611    \\
SE$^2$     &                     & 0.523       &           &          & 0.513        &             &           \\
\midrule
                          & \multicolumn{7}{c}{\textbf{Network formation model}}                                                            \\
\multicolumn{2}{l}{Same sex}                    & 0.396***    & (0.015)   & 27.043   & 0.383***     & (0.015)     & 25.850    \\
\multicolumn{2}{l}{Both Hispanic}               & 0.355***    & (0.023)   & 15.245   & 0.301***     & (0.024)     & 12.736    \\
\multicolumn{2}{l}{Both White}                  & 0.468***    & (0.022)   & 21.537   & 0.289***     & (0.024)     & 12.116    \\
\multicolumn{2}{l}{Both Black}                  & 0.859***    & (0.032)   & 26.718   & 1.117***     & (0.031)     & 36.066    \\
\multicolumn{2}{l}{Both Asian}                  & 0.164***    & (0.045)   & 3.666    & 0.290***     & (0.048)     & 6.039     \\
\multicolumn{2}{l}{Mothers education \textless High}    & 0.212***    & (0.016)   & 12.987   & 0.178***     & (0.018)     & 9.936     \\
\multicolumn{2}{l}{Mothers education \textgreater High} & 0.037**     & (0.015)   & 2.407    & 0.075***     & (0.016)     & 4.668     \\
\multicolumn{2}{l}{Mothers job Professional}       & -0.077***   & (0.017)   & -4.592   & -0.087***    & (0.019)     & -4.658    \\
\multicolumn{2}{l}{Age absolute diff}           & -0.616***   & (0.010)   & -64.156  & -0.652***    & (0.009)     & -72.445 \\
\bottomrule

\multicolumn{8}{l}{%
  \begin{minipage}{16cm}%
  \vspace{0.1cm}
    \footnotesize{Note: \textit{N} = 3,126. Observed links = 17,993. \\
    Proportion of inferred network data: censoring = 4.8\%, missing links = 76.2\%. Significance levels: $^{***} = 1$\%,   $^{**} = 5$\%, $^* = 10$\%. The explained variable is computed by taking the average grade for English, Mathematics, History, and Science, letting $A=4$, $B=3$, $C=2$, and $D=1$. Thus, lower scores indicate better academic achievement.}
  \end{minipage}%
}\\
\end{tabular} 
\end{adjustbox}

\end{table}
