# Supplementary material for: Estimating Peer Effects Using Partial Network Data
Source: arXiv:2509.08145 source file (2025-09-09)
Supplement: Supplementary file 22 [file appendix_proof.tex]

\section{Appendix -- GMM estimator: assumptions and proofs}\label{sec:appendix_proofs}

\begin{assumption}\label{as:nonsingular}
For all $s=1,...,S$ and $t=1,...,T$, $(\mathbf{I}-\alpha \dot{\mathbf{G}}^{s})$ and $(\mathbf{I}-\alpha \ddot{\mathbf{G}}^{t})$ are non-singular
\end{assumption}
In particular, when $\mathbf{G}$ is row-normalized (so $\dot{\mathbf{G}}^{s}$ and $\ddot{\mathbf{G}}^{s}$ are also row-normalized), Assumption \ref{as:alpha} implies Assumption \ref{as:nonsingular}.

We consider an objective function for the GMM estimator of the usual form: $$\textstyle\left(\frac{1}{N}\sum_i \mathbf{m}_i(\boldsymbol{\theta})\right)'\mathbf{W}_N\left(\frac{1}{N}\sum_i \mathbf{m}_i(\boldsymbol{\theta})\right),$$
where $\mathbf{m}_i(\boldsymbol{\theta})$ is the moment function.
\begin{assumption}\label{as:weigth}
$\mathbf{W}_N$ is symmetric and positive definite with $\mathbf{W}_N\rightarrow_p\mathbf{W}_0$ for $\mathbf{W}_0$ also symmetric and positive definite.
\end{assumption}

\subsection{Proof of Proposition \ref{prop:bias_nocontext}}
\noindent\textbf{Part 1: Asymptotic normality}
Define $\boldsymbol{\Delta}=\mathbf{G}-\ddot{\mathbf{G}}$ and rewrite $\boldsymbol{\eta}=\alpha[\mathbf{G}-\ddot{\mathbf{G}}]\mathbf{y}=\alpha\boldsymbol{\Delta}\mathbf{y}$. Let $\boldsymbol{\theta}_0^+ = (\boldsymbol{\theta}_0^{\prime}, 0, 0, \dots, 0)^{\prime}$ be the true value the parameter when regressors are defined as: $\ddot{\mathbf{S}}=[\mathbf{1},\mathbf{X},\mathbf{GX},\ddot{\mathbf{G}}\mathbf{X},\ddot{\mathbf{G}}\mathbf{y}]$.
The Linear GMM estimator can be written as:
\begin{align*}
    &\textstyle\hat{\boldsymbol{\theta}}=\left[\left(\frac{\ddot{\mathbf{S}}'\dot{\mathbf{Z}}}{N}\right)\mathbf{W}_N\left(\frac{\dot{\mathbf{Z}}'\ddot{\mathbf{S}}}{N}\right)\right]^{-1}\left(\frac{\ddot{\mathbf{S}}'\dot{\mathbf{Z}}}{N}\right)\mathbf{W}_N\left(\frac{\dot{\mathbf{Z}}'\ddot{\mathbf{S}}}{N}\boldsymbol{\theta}_0^+ + \frac{ \dot{\mathbf{Z}}'[\boldsymbol{\eta}+\boldsymbol{\varepsilon}]}{N}\right),\\
    &\textstyle\hat{\boldsymbol{\theta}}=\boldsymbol{\theta}_0^+ + \mathbf{M}_N\left(\frac{ \dot{\mathbf{Z}}'\boldsymbol{\eta}+\dot{\mathbf{Z}}'\boldsymbol{\varepsilon}}{N}\right),
\end{align*}
where $\textstyle\mathbf{M}_N = \left[\left(\frac{\ddot{\mathbf{S}}'\dot{\mathbf{Z}}}{N}\right)\mathbf{W}_N\left(\frac{\dot{\mathbf{Z}}'\ddot{\mathbf{S}}}{N}\right)\right]^{-1}\left(\frac{\ddot{\mathbf{S}}'\dot{\mathbf{Z}}}{N}\right)\mathbf{W}_N$.\\
Let $\textstyle\boldsymbol{\theta}^*_N =  \mathbf{M}_N\Exp\left(\frac{\dot{\mathbf{Z}}'\boldsymbol{\eta}}{N}\right)$.  Then, 
$$\textstyle
    \sqrt{N}(\hat{\boldsymbol{\theta}}-\boldsymbol{\theta}_0^+ -  \boldsymbol{\theta}^*_N) = \mathbf{M}_N N^{-1/2}\left( \dot{\mathbf{Z}}'\boldsymbol{\eta} +\dot{\mathbf{Z}}'\boldsymbol{\varepsilon} - \Exp(\dot{\mathbf{Z}}'\boldsymbol{\eta})\right).
$$
\noindent We can apply the Central Theorem Limit (CTL) to the term $N^{-1/2}\left( \dot{\mathbf{Z}}'\boldsymbol{\eta} +\dot{\mathbf{Z}}'\boldsymbol{\varepsilon} - \Exp(\dot{\mathbf{Z}}'\boldsymbol{\eta})\right)$ which can be written as $N^{-1/2}\sum_{m} \boldsymbol{\zeta}_{N,m}^{\hat{P}}$, where $\boldsymbol{\zeta}_{N,m}^{\hat{P}}$ is the sum $\dot{\mathbf{Z}}'_i\boldsymbol{\eta}_i +\dot{\mathbf{Z}}'_i\boldsymbol{\varepsilon}_i - \Exp(\dot{\mathbf{Z}}'_i\boldsymbol{\eta}_i)$ in the $m$-th sub-group. 
If the network distribution were observed, the CLT would follow directly when $M$ grows to $\infty$, because the sub-groups are independents by Assumption \ref{as:manymarkets} and then $\textstyle(\boldsymbol{\zeta}_{N,m}^{P})_m$ would be a sequence of independent variables. In the current setup, $\textstyle\boldsymbol{\zeta}_{N,m}^{\hat{P}}$'s are not independent because they all depend on $\textstyle\hat{\boldsymbol{\rho}}$ which is random. However since $\textstyle\boldsymbol{\zeta}_{N,m}^{\hat{P}} \overset{p}{\to} \boldsymbol{\zeta}_{N,m}^{P}$, then $\textstyle\boldsymbol{\zeta}_{N,m}^{\hat{P}}$'s are asymptotically independent. We use the CLT for $\ell$-\textit{mixing} array \citep[see][]{withers1981central}. Under regular conditions, in particular, $\textstyle\Var(N^{-1/2}\sum_m\boldsymbol{\zeta}_{N,m}^{\hat{P}}) < \infty$ as $M$ grows to $\infty$, the CLT implies that $\textstyle N^{-1/2}\sum_m\boldsymbol{\zeta}_{N,m}^{\hat{P}}$ converges in distribution to a $\textstyle N(\mathbf{0},\boldsymbol{\Sigma}_0)$, where
$\textstyle
\boldsymbol{\Sigma}_0= \lim_{N\to\infty}\boldsymbol{\Sigma}_N
$
and  $
\boldsymbol{\Sigma}_N= \Var(N^{-1/2}\sum_m\boldsymbol{\zeta}_{N,m}^{\hat{P}})
$.\\
\noindent $\boldsymbol{\Sigma}_0$ can be estimated by $\boldsymbol{\Sigma}_N$, where
\begin{align}
   \textstyle \boldsymbol{\Sigma}_N &=\textstyle \Exp(\Var(N^{-1/2}\sum_m\boldsymbol{\zeta}_{N,m}^{\hat{P}}|{\hat{P}})) + \Var(\Exp(N^{-1/2}\sum_m\boldsymbol{\zeta}_{N,m}^{\hat{P}}|{\hat{P}})), \nonumber\\
   \textstyle \boldsymbol{\Sigma}_N &=\textstyle N^{-1}\Exp(\sum_m\Var(\boldsymbol{\zeta}_{N,m}^{\hat{P}}|{\hat{P}})) + N^{-1}\Var(\sum_m\Exp(\boldsymbol{\zeta}_{N,m}^{\hat{P}}|{\hat{P}})). \nonumber
\end{align}
The term $\textstyle N^{-1}\Exp(\sum_m\Var(\boldsymbol{\zeta}_{N,m}^{\hat{P}}|{\hat{P}}))$ is due to the error term of the model $\textstyle\boldsymbol{\varepsilon}$ and the fact that the true network is not observed whereas $\textstyle N^{-1}\Var(\sum_m\Exp(\boldsymbol{\zeta}_{N,m}^{\hat{P}}|{\hat{P}}))$ is due to uncertainty associated with the estimation of $P$.\\
Besides, by the law of large numbers (LLN), $\textstyle\mathbf{M}_N \overset{p}{\to} \mathbf{M}_0$. As a result,
\begin{equation}
    \sqrt{N}(\hat{\boldsymbol{\theta}}-\boldsymbol{\theta}_0^++ \boldsymbol{\theta}_N^*) \overset{d}{\to} N(0, \mathbf{M}_0\boldsymbol{\Sigma}_0\mathbf{M}_0^{\prime}). \label{eq:asym:iv}
\end{equation}
\noindent The asymptotic bias of $\hat{\boldsymbol{\theta}}$ is then given by $\textstyle \plim \boldsymbol{\theta}_N^{\ast} = \alpha \mathbf{M}_0 \plim[\dot{\mathbf{Z}}'({\mathbf{G}}-\ddot{\mathbf{G}})\mathbf{y}/N]$.

\noindent\textbf{Part 2: Choice of $\mathbf{W}$}
Let $\mathbf{K}=\dot{\mathbf{Z}}'\boldsymbol{\Delta}\mathbf{G}^2/N$ if $\boldsymbol{\gamma}=\mathbf{0}$ and $\mathbf{K}=\dot{\mathbf{Z}}'\boldsymbol{\Delta}/N$ otherwise. Consider $\Vert \mathbf{MK}\Vert_F=\sqrt{trace(\mathbf{K}'\mathbf{M}'\mathbf{M}\mathbf{K})}=\sqrt{trace(\mathbf{K}\mathbf{K}'\mathbf{M}'\mathbf{M})}$. We have:
$$
(1/N^2)\mathbf{M}\mathbf{M}'=[\ddot{\mathbf{S}}'\dot{\mathbf{Z}}\mathbf{W}\dot{\mathbf{Z}}'\ddot{\mathbf{S}}]^{-1}\ddot{\mathbf{S}}'\dot{\mathbf{Z}}\mathbf{W}\mathbf{W}\dot{\mathbf{Z}}'\ddot{\mathbf{S}}[\ddot{\mathbf{S}}'\dot{\mathbf{Z}}\mathbf{W}\dot{\mathbf{Z}}'\ddot{\mathbf{S}}]^{-1}
$$
Let $\mathbf{W}=\mathbf{C}'\mathbf{C}$ and let $\mathbf{B}=\ddot{\mathbf{S}}'\dot{\mathbf{Z}}\mathbf{C}'$. We have:
$$
(1/N^2)\mathbf{M}\mathbf{M}'=(\mathbf{B}'\mathbf{B})^{-1}\mathbf{B}'\mathbf{C}\mathbf{C}'
\mathbf{B}(\mathbf{B}'\mathbf{B})^{-1}
$$
Now, define $\mathbf{J}'=(\mathbf{B}'\mathbf{B})^{-1}\mathbf{B}'\mathbf{C}-(\mathbf{B}'(\mathbf{C}')^{-1}\mathbf{C}^{-1}\mathbf{B})^{-1}\mathbf{B}'(\mathbf{C}')^{-1}$. We have:
$$
(1/N^2)\mathbf{M}\mathbf{M}'=\mathbf{J}'\mathbf{J}+(\mathbf{B}'(\mathbf{C}')^{-1}\mathbf{C}^{-1}\mathbf{B})^{-1}=\mathbf{J}'\mathbf{J}+ (\ddot{\mathbf{S}}'\dot{\mathbf{Z}}\dot{\mathbf{Z}}'\ddot{\mathbf{S}})^{-1}
$$
Therefore, we have:
$$
(1/N^2)\Vert \mathbf{M}\Vert_F=\sqrt{trace(\mathbf{J}'\mathbf{J}+ (\ddot{\mathbf{S}}'\dot{\mathbf{Z}}\dot{\mathbf{Z}}'\ddot{\mathbf{S}})^{-1})}=\sqrt{trace(\mathbf{J}'\mathbf{J})+ trace((\ddot{\mathbf{S}}'\dot{\mathbf{Z}}\dot{\mathbf{Z}}'\ddot{\mathbf{S}})^{-1})}
$$
When $\mathbf{W}=\mathbf{I}$, we have that $\mathbf{J}=\mathbf{0}$ and the Frobenius norm of $\mathbf{M}$ is given by $N^2\sqrt{trace((\ddot{\mathbf{S}}'\dot{\mathbf{Z}}\dot{\mathbf{Z}}'\ddot{\mathbf{S}})^{-1})}$.

\subsection{Proof of Theorem \ref{prop:non_observed}}
\subsubsection{Validity of the moment condition and consistency}
Let $$\textstyle\mathbf{m}_i(\boldsymbol{\theta})=\frac{1}{ST}\sum_s\sum_t\dot{\mathbf{Z}}_i^{(s)\prime}(\mathbf{I}-\alpha\dot{\mathbf{G}}^{(s)})_i\left(\mathbf{y}-(\mathbf{I}-\alpha\ddot{\mathbf{G}}^{(t)})^{-1}\ddot{\mathbf{V}}^{(t)}\tilde{\boldsymbol{\theta}}\right)$$

By construction, we have: $\textstyle\plim\mathbb{E}\left(\mathbf{m}_i(\boldsymbol{\theta})\right)=\mathbf{0}$ for any finite $S$ and $T$.

To see why, lets substitute $\mathbf{y}=(\mathbf{I}-\alpha\mathbf{G})^{-1}(\mathbf{V}\tilde{\boldsymbol{\theta}}+\boldsymbol{\varepsilon})$ in the moment function. We have:
\begin{eqnarray*}
\textstyle\mathbf{m}_i(\boldsymbol{\theta})&=&\textstyle\frac{1}{ST}\sum_s\sum_t \dot{\mathbf{Z}}_i^{(s)\prime}(\mathbf{I}-\alpha\dot{\mathbf{G}}^{(s)})_i\left[(\mathbf{I}-\alpha\mathbf{G})^{-1}\mathbf{V}-(\mathbf{I}-\alpha\ddot{\mathbf{G}}^{(t)})^{-1}\ddot{\mathbf{V}}^{(t)}\right]\tilde{\boldsymbol{\theta}}\\
&+&\textstyle\frac{1}{S}\sum_s \dot{\mathbf{Z}}_i^{(s)\prime}(\mathbf{I}-\alpha\dot{\mathbf{G}}^{(s)})_i(\mathbf{I}-\alpha\mathbf{G})^{-1}\boldsymbol{\varepsilon}
\end{eqnarray*}
It is therefore sufficient that for any $s,t$:
$$\textstyle
\mathbb{E}\left(\dot{\mathbf{Z}}_i^{(s)\prime}(\mathbf{I}-\alpha\dot{\mathbf{G}}^{(s)})_i(\mathbf{I}-\alpha\mathbf{G})^{-1}\boldsymbol{\varepsilon}\right)=\mathbf{0},
$$
which holds directly from Assumption \ref{as:alpha} and the specification of the network formation process (see Assumption \ref{as:partial}), and that
$$\textstyle
\plim \mathbb{E}\left[\dot{\mathbf{Z}}_i^{(s)\prime}(\mathbf{I}-\alpha\dot{\mathbf{G}}^{(s)})_i\left[(\mathbf{I}-\alpha\mathbf{G})^{-1}\mathbf{V}-(\mathbf{I}-\alpha\ddot{\mathbf{G}}^{(t)})^{-1}\ddot{\mathbf{V}}^{(t)}\right]\tilde{\boldsymbol{\theta}}\right]=\mathbf{0},
$$
where $\plim$ is the probability limit. \\
Note that, for N fixed, $\mathbf{G}$, $\dot{\mathbf{G}}^{(s)}$, and $\ddot{\mathbf{G}}^{(t)}$ have a finite number of possible realizations. Thus, $\textstyle\mathbb{E}\left[\dot{\mathbf{Z}}_i^{(s)\prime}(\mathbf{I}-\alpha\dot{\mathbf{G}}^{(s)})_i(\mathbf{I}-\alpha\mathbf{G})^{-1}\mathbf{V}\tilde{\boldsymbol{\theta}}\right]$ can be written as a continuous function of $P$, the distribution of the adjacency matrix, and $\hat{P}$, a consistent estimator of that distribution.\footnote{The function would essentially composed of summations and products of terms depending on $P$ and $\hat{P}$.} Analogously, $\mathbb{E}\left[\dot{\mathbf{Z}}_i^{(s)\prime}(\mathbf{I}-\alpha\dot{\mathbf{G}}^{(s)})_i(\mathbf{I}-\alpha\ddot{\mathbf{G}}^{(t)})^{-1}\ddot{\mathbf{V}}^{(t)}\tilde{\boldsymbol{\theta}}\right]$ also can be written as a same function with the difference that $P$ is replaced by $\hat{P}$. As both functions are continuous and since $\hat{P}$ converges in probability to $P$ (see Assumption \ref{as:partial}), their limits are obtained by replacing $\hat{P}$ by $P$ and then equal. As such, we have:
$$
\plim \mathbb{E}\left[\dot{\mathbf{Z}}_i^{(s)\prime}(\mathbf{I}-\alpha\dot{\mathbf{G}}^{(s)})_i(\mathbf{I}-\alpha\mathbf{G})^{-1}\mathbf{V}\tilde{\boldsymbol{\theta}}\right]=\plim \mathbb{E}\left[\dot{\mathbf{Z}}_i^{(s)\prime}(\mathbf{I}-\alpha\dot{\mathbf{G}}^{(s)})_i(\mathbf{I}-\alpha\ddot{\mathbf{G}}^{(t)})^{-1}\ddot{\mathbf{V}}^{(t)}\tilde{\boldsymbol{\theta}}\right].
$$

\noindent The GMM estimator
$$\textstyle
\hat{\boldsymbol{\theta}}=\arg\max \left(\frac{1}{N}\sum_i\mathbf{m}_i(\boldsymbol{\theta})\right)'\mathbf{W}_N\left(\frac{1}{N}\sum_i\mathbf{m}_i(\boldsymbol{\theta})\right)
$$
is therefore consistent under Assumptions \ref{as:manymarkets}-\ref{as:weigth} and an identification condition, which we now discuss.

\subsubsection{Concentration and Identification\label{app:ident}}
While the GMM estimator could be solved numerically, it is helpful to concentrate the objective function around $\alpha$.
Let $\textstyle\mathbf{R}(\alpha)=\frac{1}{ST}\sum_s\sum_t\dot{\mathbf{Z}}^{(s)\prime}(\mathbf{I}-\alpha\dot{\mathbf{G}}^{(s)})(\mathbf{I}-\alpha\ddot{\mathbf{G}}^{(t)})^{-1}\ddot{\mathbf{V}}^{(t)}$ and $\textstyle\mathbf{D}(\alpha)=\frac{1}{ST}\sum_s\sum_t\dot{\mathbf{Z}}^{(s)\prime}(\mathbf{I}-\alpha\dot{\mathbf{G}}^{(s)})$ so that $\textstyle\frac{1}{N}\sum_i\mathbf{m}_i(\boldsymbol{\theta})=\mathbf{D}(\alpha)\mathbf{y}-\mathbf{R}(\alpha)\tilde{\boldsymbol{\theta}}$.

The gradient of the objective function with respect to $\textstyle\tilde{\boldsymbol{\theta}}$ is:
$$
\textstyle-2\left(\frac{1}{N}\mathbf{D}(\alpha)\mathbf{y}-\mathbf{R}(\alpha)\tilde{\boldsymbol{\theta}}\right)'\mathbf{W}_N\mathbf{R(\alpha)}.
$$
The hessian is therefore: $\mathbf{R}'(\alpha)\mathbf{W}_N\mathbf{R(\alpha)}$ which is semi-positive definite. Hence, the following assumption ensures identification of $\tilde{\boldsymbol{\theta}}$, conditional on $\alpha$.

\begin{assumption}\label{as:convex}
$\mathbf{R}'(\alpha)\mathbf{W}_N\mathbf{R(\alpha)}$ is non-singular for all $\alpha$.
\end{assumption}
\noindent A sufficient condition is that $\mathbf{R}'(\alpha)$ has full rank, for all $\alpha$.\\
Under Assumption \ref{as:convex}, the estimator of $\tilde{\boldsymbol{\theta}}$ conditionally on $\alpha$ is\\ $\hat{\tilde{\boldsymbol{\theta}}}(\alpha)=(\mathbf{R}'(\alpha)\mathbf{W}_N\mathbf{R(\alpha)})^{-1}\mathbf{R}'(\alpha)\mathbf{W}_N\mathbf{D}(\alpha)\mathbf{y}$.\\
The objective function can then be concentrated around $\alpha$, as 
$$\textstyle
\left(\frac{1}{N}\mathbf{D}(\alpha)\mathbf{y}-\mathbf{R}(\alpha)\hat{\tilde{\boldsymbol{\theta}}}(\alpha)\right)'\mathbf{W}_N\left(\frac{1}{N}\mathbf{D}(\alpha)\mathbf{y}-\mathbf{R}(\alpha)\hat{\tilde{\boldsymbol{\theta}}}(\alpha)\right).
$$
While we cannot easily ensure that this function is globally convex in $\alpha$, the behavior of the function is easy to study since $\alpha$ is uni-dimensional and has a bounded support (see Assumption \ref{as:alpha}). Note that numerically minimizing the concentrated objective function implicitly checks Assumption \ref{as:convex}. Our final assumption ensures identification of $\alpha$.
\begin{assumption}
The concentrated objective function admits an interior global minimum.
\end{assumption}

\subsubsection{Asymptotic Normality}
The moment function depends on $\hat P$, the estimated distribution of the network. For the sake of clarification in this section, we write the moment function as $\mathbf{m}_i^{\hat{P}}(\boldsymbol{\theta})$ instead of $\mathbf{m}_i(\boldsymbol{\theta})$. This allows to distinguish $\mathbf{m}_i^{\hat{P}}(\boldsymbol{\theta})$, the biased (but consistent) moment function we use, from  $\mathbf{m}_i^{P}(\boldsymbol{\theta})$ which is the unbiased moment function we would use if the true distribution of $\mathbf{G}$ were known.\\
Taking the first derivative of the objective function with respect to $\boldsymbol{\theta}$, we have:
$$\textstyle
\frac{1}{N}\sum_i\frac{\partial\mathbf{m}_i^{\hat{P}}(\boldsymbol{\theta})^{\prime}}{\partial\boldsymbol{\theta}}\mathbf{W}_N\frac{1}{N}\sum_i\mathbf{m}_i^{\hat{P}}(\boldsymbol{\theta})=\mathbf{0}.
$$
By applying the mean value theorem to $\frac{1}{N}\sum_i\mathbf{m}_i^{\hat{P}}(\boldsymbol{\theta})$, we have:

$$\textstyle\sqrt{N}(\hat{\boldsymbol{\theta}}-\boldsymbol{\theta}_0)=-\left[\frac{1}{N}\sum_i\frac{\partial\mathbf{m}_i^{\hat{P}}(\hat{\boldsymbol{\theta}})^{\prime}}{\partial\boldsymbol{\theta}} \mathbf{W}_N \frac{1}{N}\sum_i\frac{\partial\mathbf{m}_i^{\hat{P}}({\boldsymbol{\theta}^*})}{\partial\boldsymbol{\theta}^{\prime}}\right]^{-1}\frac{1}{N}\sum_i\frac{\partial\mathbf{m}_i^{\hat{P}}(\hat{\boldsymbol{\theta}})^{\prime}}{\partial\boldsymbol{\theta}} \mathbf{W}_NN^{-1/2}\sum_i\mathbf{m}_i^{\hat{P}}(\boldsymbol{\theta}_0),   $$
where $\boldsymbol{\theta}^*$ is between $\hat{\boldsymbol{\theta}}$ and $\boldsymbol{\theta}_0$.  \\
Let $$\textstyle\mathbf{H}_N = \left[\frac{1}{N}\sum_i\frac{\partial\mathbf{m}_i^{\hat{P}}(\hat{\boldsymbol{\theta}})^{\prime}}{\partial\boldsymbol{\theta}} \mathbf{W}_N \frac{1}{N}\sum_i\frac{\partial\mathbf{m}_i^{\hat{P}}({\boldsymbol{\theta}^*})}{\partial\boldsymbol{\theta}^{\prime}}\right]^{-1}\frac{1}{N}\sum_i\frac{\partial\mathbf{m}_i^{\hat{P}}(\hat{\boldsymbol{\theta}})^{\prime}}{\partial\boldsymbol{\theta}} \mathbf{W}_N$$
and 
\begin{equation}\label{eq:thetastar}\textstyle
    \boldsymbol{\theta}_N^* = \frac{1}{N}\mathbf{H}_N \sum_i\Exp(\mathbf{m}_i^{\hat{P}}(\boldsymbol{\theta}_0)).
\end{equation}
We have $$\textstyle\sqrt{N}(\hat{\boldsymbol{\theta}}-\boldsymbol{\theta}_0 + \boldsymbol{\theta}_N^* )=-\mathbf{H}_NN^{-1/2}\sum_i\Tilde{\mathbf{m}}_i^{\hat{P}}(\boldsymbol{\theta}_0),$$
where $\Tilde{\mathbf{m}}_i^{\hat{P}}(\boldsymbol{\theta}_0) = \mathbf{m}_i^{\hat{P}}(\boldsymbol{\theta}_0) - \Exp(\mathbf{m}_i^{\hat{P}}(\boldsymbol{\theta}_0))$. Note that $\boldsymbol{\theta}_N^* \overset{p}{\to} \mathbf{0}$ since $\hat{P}$ is consistent.\\
Let $\boldsymbol{\zeta}_{N,m}^{\hat{P}}$ be the sum of $\tilde{\mathbf{m}}_i^{\hat{P}}(\boldsymbol{\theta}_0)$ over the $m$-th sub-network and let $\boldsymbol{\zeta}_{N,m}^{P}$ be the same statistic where $\hat{P}$ is replaced by $P$. We have $\textstyle\sum_i\tilde{\mathbf{m}}_i^{\hat{P}}(\boldsymbol{\theta}_0)  = \sum_m \boldsymbol{\zeta}_{N,m}^{\hat{P}}$. We need to apply the Central Limit Theorem (CLT) to $N^{-1/2}\sum_m \boldsymbol{\zeta}_{N,m}^{\hat{P}}$. If the network distribution were observed, the CLT would follow directly when $M$ grows to $\infty$, because the sub-groups are independents by Assumption \ref{as:manymarkets} and then $\textstyle(\boldsymbol{\zeta}_{N,m}^{P})_m$ would be a sequence of independent variables. In the current setup, $\textstyle\boldsymbol{\zeta}_{N,m}^{\hat{P}}$'s are not independent because they all depend on $\textstyle\hat{\boldsymbol{\rho}}$ which is random. However since $\textstyle\boldsymbol{\zeta}_{N,m}^{\hat{P}} \overset{p}{\to} \boldsymbol{\zeta}_{N,m}^{P}$, then $\textstyle\boldsymbol{\zeta}_{N,m}^{\hat{P}}$'s are asymptotically independent. We use the CLT for $\ell$-\textit{mixing} array \citep[see][]{withers1981central}. Under regular conditions, in particular, $\textstyle\Var(N^{-1/2}\sum_m\boldsymbol{\zeta}_{N,m}^{\hat{P}}) < \infty$ as $M$ grows to $\infty$, the CLT implies that $\textstyle N^{-1/2}\sum_m\boldsymbol{\zeta}_{N,m}^{\hat{P}}$ converges in distribution to a $\textstyle N(\mathbf{0},\boldsymbol{\Sigma}_0)$, where
$\textstyle
\boldsymbol{\Sigma}_0= \lim_{N\to\infty}\boldsymbol{\Sigma}_N
$
and  $\textstyle
\boldsymbol{\Sigma}_N= \Var(N^{-1/2}\sum_m\boldsymbol{\zeta}_{N,m}^{\hat{P}})
$.\\
In addition to the uncertainty due to $\boldsymbol{\varepsilon}$, the variance $\boldsymbol{\Sigma}_0$ includes uncertainty due to $\hat{\boldsymbol{\rho}}$ which is prior estimated using a network formation model.\\
Besides, by the law of large numbers (LLN), $\textstyle\dfrac{1}{N}\sum_i\dfrac{\partial\mathbf{m}_i^{\hat{P}}(\hat{\boldsymbol{\theta}})^{\prime}}{\partial\boldsymbol{\theta}} \overset{p}{\to} \boldsymbol{\Delta}m_0^{P} = \Exp(\dfrac{\partial\mathbf{m}_i^{\hat{P}}(\hat{\boldsymbol{\theta}})^{\prime}}{\partial\boldsymbol{\theta}})$. Thus $\textstyle\mathbf{H}_N \overset{p}{\to} \mathbf{H}_0 = (\boldsymbol{\Delta}\mathbf{m}_0^{P}\mathbf{W}_0 \boldsymbol{\Delta}\mathbf{m}_0^{P\prime})^{-1}\boldsymbol{\Delta}\mathbf{m}_0^{P}\mathbf{W}_0$. As a result,
\begin{equation}\textstyle
    \sqrt{N}(\hat{\boldsymbol{\theta}}-\boldsymbol{\theta}_0 + \boldsymbol{\theta}_N^*) \overset{d}{\to} N(0, \mathbf{H}_0\boldsymbol{\Sigma}_0\mathbf{H}_0^{\prime}).
\end{equation}
\noindent This result implies that $\hat{\boldsymbol{\theta}}$ is not $\sqrt{N}$-consistent to $\boldsymbol{\theta}_0$. However, as $\lim_{N\to\infty}\boldsymbol{\theta}_N^* = 0$, $\hat{\boldsymbol{\theta}}$ is consistent.\footnote{In addition, if $\lim_{N\to\infty}\sqrt{N}\boldsymbol{\theta}_N^* = o_p(1)$, then $\sqrt{N}(\hat{\boldsymbol{\theta}}-\boldsymbol{\theta}_0) \overset{d}{\to} N(0, \mathbf{H}_0\boldsymbol{\Sigma}_0\mathbf{H}_0^{\prime}).$} This result is sufficient to perform statistical tests on $\boldsymbol{\theta}_0$ when $M$ is large since the asymptotic distribution of $\hat{\boldsymbol{\theta}}$ is  $N(\boldsymbol{\theta}_0 - \boldsymbol{\theta}_N^*, \Var(\hat{\boldsymbol{\theta}}))$, where $\boldsymbol{\theta}_N^*$ is approximately equal to zero and asymptotic variance is
\begin{equation}\textstyle
    \Var(\hat{\boldsymbol{\theta}}) = \dfrac{\mathbf{H}_0\boldsymbol{\Sigma}_0\mathbf{H}_0^{\prime}}{N}\label{var:gmm}
\end{equation}
On the one hand, $\mathbf{H}_0$ can be estimated consistently by, $$\textstyle\hat{\mathbf{H}}_0 = N\left[\sum_i\dfrac{\partial\mathbf{m}_i^{\hat{P}}(\hat{\boldsymbol{\theta}})^{\prime}}{\partial\boldsymbol{\theta}} \mathbf{W}_N \sum_i\dfrac{\partial\mathbf{m}_i^{\hat{P}}({\hat{\boldsymbol{\theta}}})}{\partial\boldsymbol{\theta}^{\prime}}\right]^{-1}\sum_i\dfrac{\partial\mathbf{m}_i^{\hat{P}}(\hat{\boldsymbol{\theta}})^{\prime}}{\partial\boldsymbol{\theta}} \mathbf{W}_N.$$
\noindent On the other hand, $\boldsymbol{\Sigma}_0$ can be estimated by $\boldsymbol{\Sigma}_N$, where
\begin{align}
    \textstyle\boldsymbol{\Sigma}_N &=\textstyle \Exp(\Var(N^{-1/2}\sum_m\boldsymbol{\zeta}_{N,m}^{\hat{P}}|{\hat{P}})) + \Var(\Exp(N^{-1/2}\sum_m\boldsymbol{\zeta}_{N,m}^{\hat{P}}|{\hat{P}})), \nonumber\\
    \textstyle\boldsymbol{\Sigma}_N &=\textstyle N^{-1}\Exp(\sum_m\Var(\boldsymbol{\zeta}_{N,m}^{\hat{P}}|{\hat{P}})) + N^{-1}\Var(\sum_m\Exp(\boldsymbol{\zeta}_{N,m}^{\hat{P}}|{\hat{P}})). \nonumber
\end{align}
The term $\textstyle N^{-1}\Exp(\sum_m\Var(\boldsymbol{\zeta}_{N,m}^{\hat{P}}|{\hat{P}}))$ is due to the error term of the model $\boldsymbol{\varepsilon}$ and the fact that the true network is not observed whereas $\textstyle N^{-1}\Var(\sum_m\Exp(\boldsymbol{\zeta}_{N,m}^{\hat{P}}|{\hat{P}}))$ is due to uncertainty associated with the estimation of $P$.
In practice we estimate, we can compute the estimator of $\textstyle \boldsymbol{\zeta}_{N,m}^{\hat{P}}$, $m = 1, ~\to, M$. Thus, we can also estimate $\textstyle \sum_m\Var(\boldsymbol{\zeta}_{N,m}^{\hat{P}}|{\hat{P}})$ and $\textstyle \sum_m\Exp(\boldsymbol{\zeta}_{N,m}^{\hat{P}}|{\hat{P}})$. With several simulations from the distribution of $\hat{P}$, we finally compute $\boldsymbol{\Sigma}_N$.\footnote{Our R package offers tools to compute this variance. See also our online appendix.}

\subsection{Additional Results}

\subsubsection{Bias correction for $\mathbf{GX}$ observed}

Let us replace $\ddot{\mathbf{V}}$ with $\mathbf{V}$ in (\ref{eq:bias_corr}). We have:
$$
\dot{\mathbf{Z}}^{(r)\prime}_i\left[(\mathbf{I}-\alpha\dddot{\mathbf{G}}^{(t)})_i\left((\mathbf{I}-\alpha{\mathbf{G}})^{-1}-(\mathbf{I}-\alpha\ddot{\mathbf{G}}^{(s)})^{-1}\right)\mathbf{V}\tilde{\boldsymbol{\theta}}\right]
$$
which is equal to:
$$
\dot{\mathbf{Z}}^{(r)\prime}_i\left[(\mathbf{I}-\alpha\dddot{\mathbf{G}}^{(t)})_i\left((\mathbf{I}-\alpha{\mathbf{G}})^{-1}-(\mathbf{I}-\alpha\ddot{\mathbf{G}}^{(s)})^{-1}\right)\left((\mathbf{I}-\alpha\mathbf{G})\mathbf{y} + \boldsymbol{\varepsilon}\right)\right]
%\mathbb{E}\dot{\mathbf{Z}}(\mathbf{I}-\alpha\dddot{\mathbf{G}})(\mathbf{I}-\alpha\ddot{\mathbf{G}})^{-1}(\mathbf{I}-\alpha\ddot{\mathbf{G}})[(\mathbf{I}-\alpha{\mathbf{G}})^{-1}-(\mathbf{I}-\alpha\ddot{\mathbf{G}})^{-1}](\mathbf{I}-\alpha{\mathbf{G}})(\mathbf{I}-\alpha{\mathbf{G}})^{-1}\mathbf{V}\tilde{\boldsymbol{\theta}}
$$
which simplifies to:
$$
\dot{\mathbf{Z}}^{(r)\prime}_i(\mathbf{I}-\alpha\dddot{\mathbf{G}}^{(t)})_i(\mathbf{I}-\alpha\ddot{\mathbf{G}}^{(s)})^{-1}[\alpha({\mathbf{G}}-\ddot{\mathbf{G}}^{(s)})]\mathbf{y} + \dot{\mathbf{Z}}^{(r)\prime}_i\left[(\mathbf{I}-\alpha\dddot{\mathbf{G}}^{(t)})_i\left((\mathbf{I}-\alpha{\mathbf{G}})^{-1}-(\mathbf{I}-\alpha\ddot{\mathbf{G}}^{(s)})^{-1}\right)\boldsymbol{\varepsilon}\right]
$$
\noindent Note that the expectation of the term $\dot{\mathbf{Z}}^{(r)\prime}_i\left[(\mathbf{I}-\alpha\dddot{\mathbf{G}}^{(t)})_i\left((\mathbf{I}-\alpha{\mathbf{G}})^{-1}-(\mathbf{I}-\alpha\ddot{\mathbf{G}}^{(s)})^{-1}\right)\boldsymbol{\varepsilon}\right]$  is null.

\subsubsection{Corollaries}
\begin{corollary}\label{prop:GXobs}
Assume that $\mathbf{GX}$ is observed, but that $\mathbf{Gy}$ is not observed. Let $\dot{\mathbf{Z}}^{(s)}=[\mathbf{1},\mathbf{X},{\mathbf{G}}\mathbf{X},\dot{\mathbf{G}}^{s}{\mathbf{G}}\mathbf{X},(\dot{\mathbf{G}}^{(s)})^2{\mathbf{G}}\mathbf{X},...]$,
$\ddot{\mathbf{Z}}^{(s,t)}=[\mathbf{1},\mathbf{X},\ddot{\mathbf{G}}^{(t)}\mathbf{X},\dot{\mathbf{G}}^{s}\ddot{\mathbf{G}}^{(t)}\mathbf{X},(\dot{\mathbf{G}}^{(s)})^2\ddot{\mathbf{G}}^{(t)}\mathbf{X},...]$, $\mathbf{V}=[\mathbf{1},\mathbf{X},\mathbf{G}\mathbf{X}]$, and $\ddot{\mathbf{V}}^{(t)}=[\mathbf{1},\mathbf{X},\ddot{\mathbf{G}}^{(t)}\mathbf{X}]$. Then, the results from Theorem \ref{prop:non_observed} hold for the following (simulated) moment function:
\begin{eqnarray}\label{eq:Gyobs}
\frac{1}{S}\sum_{s=1}^S\dot{\mathbf{Z}}_i^{(s)\prime}(\mathbf{I}-\alpha\dot{\mathbf{G}}^{(s)})_i\mathbf{y} -
\frac{1}{ST}\sum_{t=1}^T\sum_{s=1}^S (\dot{\mathbf{Z}}^{(s)\prime}\mathbf{V}-\ddot{\mathbf{Z}}^{(s,t)\prime}\ddot{\mathbf{V}}^{(t)})_i\tilde{\boldsymbol{\theta}}\nonumber\\ -\frac{1}{ST}\sum_{t=1}^T\sum_{s=1}^S  \ddot{\mathbf{Z}}^{(s,t)\prime}_i(\mathbf{I}-\alpha\dot{\mathbf{G}}^{(s)})_i(\mathbf{I}-\alpha\ddot{\mathbf{G}}^{(t)})^{-1}\ddot{\mathbf{V}}^{(t)}\tilde{\boldsymbol{\theta}}
\end{eqnarray}
\end{corollary}

\begin{corollary}\label{prop:Gyobs}
Assume that $\mathbf{Gy}$ is observed, but that $\mathbf{GX}$ is not observed. Let $\dot{\mathbf{Z}}^{(s)}=[\mathbf{1},\mathbf{X},\dot{\mathbf{G}}^{(s)}\mathbf{X},(\dot{\mathbf{G}}^{(s)})^2\mathbf{X},...]$, and $\ddot{\mathbf{V}}^{(t)}=[\mathbf{1},\mathbf{X},\ddot{\mathbf{G}}^{(t)}\mathbf{X}]$.  Then, the results from Theorem \ref{prop:non_observed} hold for the following (simulated) moment function:
\begin{eqnarray}\label{eq:GXobs}
\frac{1}{S}\sum_{s=1}^S\dot{\mathbf{Z}}_i^{(s)\prime}(\mathbf{I}-\alpha\mathbf{G})_i\mathbf{y} -
\frac{1}{ST}\sum_{t=1}^T\sum_{s=1}^S \dot{\mathbf{Z}}^{(s)\prime}_i\ddot{\mathbf{V}}^{(t)}_i\tilde{\boldsymbol{\theta}}
\end{eqnarray}
\end{corollary}
