# Supplementary material for: Estimating Peer Effects Using Partial Network Data
Source: arXiv:2509.08145 source file (2025-09-09)
Supplement: Supplementary file 25 [file appendix_backup.tex]

\section{Appendix -- Supplementary Material}
\subsection{Additional Monte-Carlo Results}\label{sec:addmontecarlo}

\begin{table}[!htbp] 
\centering
\caption{Simulation results without contextual effects (2).} 
\label{tab:simple2} 
\begin{tabular}{@{\extracolsep{5pt}}ld{4}d{4}d{4}d{4}d{4}} 
\\[-1.8ex]\hline 
\hline \\[-1.8ex] 
Statistic & \multicolumn{1}{c}{Mean} & \multicolumn{1}{c}{Std. Dev.} & \multicolumn{1}{c}{Pctl(25)} & \multicolumn{1}{c}{Median} & \multicolumn{1}{c}{Pctl(75)} \\ 
\hline\hline \\[-1.8ex] 
\multicolumn{6}{c}{$N=50$, $M=100$ - $\mathbf{Gy}$ \textbf{is Observed}}\\\hline \\[-1.8ex] 
\multicolumn{6}{c}{Estimation results}\\\hline\\[-1.8ex] 
$Intercept=2$ & 2.011 & 0.263 & 1.844 & 2.007 & 2.182 \\
$\alpha=0.4$ & 0.399 & 0.014 & 0.390 & 0.400 & 0.409 \\
$\beta_1=1$  & 1.000 & 0.003 & 0.998 & 1.000 & 1.002 \\
$\beta_2=1.5$   & 1.500 & 0.006 & 1.496 & 1.500 & 1.504 \\
\hline\\[-1.8ex] 
\multicolumn{6}{c}{Tests}\\\hline\\[-1.8ex] 
\textit{F}-test & 1302.788 & 232.211 & 1145.790 & 1289.808 & 1445.453 \\
Hausman  & 1.210 & 1.713 & 0.099 & 0.509 & 1.642 \\
Sargan & 0.970 & 1.382 & 0.095 & 0.420 & 1.300 \\
\hline\hline\\[-1.8ex] 
\multicolumn{6}{c}{$N=50$, $M=100$ - $\mathbf{Gy}$ \textbf{is not observed - same draw}}\\\hline\\[-1.8ex] 
\multicolumn{6}{c}{Estimation results}\\\hline\\[-1.8ex] 
$Intercept=2$ & 4.843 & 0.324 & 4.630 & 4.828 & 5.044 \\
$\alpha=0.4$ & 0.244 & 0.017 & 0.234 & 0.245 & 0.256 \\
$\beta_1=1$ & 1.002 & 0.003 & 1.000 & 1.002 & 1.004 \\
$\beta_2=1.5$ & 1.503 & 0.007 & 1.498 & 1.503 & 1.507 \\
\hline\\[-1.8ex] 
\multicolumn{6}{c}{Tests}\\\hline\\[-1.8ex] 
\textit{F}-test & 26588.232 & 2113.817 & 25076.054 & 26534.073 & 27959.250 \\
Hausman & 339.782 & 44.092 & 310.264 & 338.783 & 368.245 \\
Sargan & 2.261 & 3.229 & 0.237 & 1.067 & 3.085 \\
\hline \\[-1.8ex] 
\multicolumn{6}{c}{Validity}\\\hline\\[-1.8ex] 
$cor(\eta_i,\hat{x}_{i,1})$ & -0.403 & 0.019 & -0.416 & -0.403 & -0.390 \\
$cor(\eta_i,\hat{x}_{i,2})$  & -0.296 & 0.017 & -0.307 & -0.296 & -0.284 \\
\hline\hline\\[-1.8ex] 
\multicolumn{6}{c}{$N=50$, $M=100$ - $\mathbf{Gy}$ \textbf{is not observed - different draws}}\\\hline\\[-1.8ex] 
\multicolumn{6}{c}{Estimation results}\\\hline\\[-1.8ex] 
$Intercept=2$ & 2.018 & 0.302 & 1.828 & 2.020 & 2.213 \\
$\alpha=0.4$ & 0.399 & 0.016 & 0.389 & 0.399 & 0.409 \\
$\beta_1=1$ & 1.000 & 0.003 & 0.998 & 1.000 & 1.002 \\
$\beta_2=1.5$ & 1.500 & 0.007 & 1.495 & 1.500 & 1.505 \\
\hline \\[-1.8ex] 
\multicolumn{6}{c}{Tests}\\\hline\\[-1.8ex] 
\textit{F}-test & 1311.739 & 231.331 & 1150.204 & 1305.262 & 1457.470 \\
Hausman & 71.466 & 18.214 & 58.611 & 70.960 & 82.160 \\
Sargan & 1.000 & 1.365 & 0.095 & 0.456 & 1.389 \\
\hline \\[-1.8ex] 
\multicolumn{6}{c}{Validity}\\\hline\\[-1.8ex] 
$cor(\eta_i,\hat{x}_{i,1})$ & -0.001 & 0.015 & -0.011 & 0.000 & 0.009 \\
$cor(\eta_i,\hat{x}_{i,2})$ & -0.001 & 0.014 & -0.010 & -0.001 & 0.009 \\
\hline \\[-1.8ex] \\
\multicolumn{6}{l}{%
  \begin{minipage}{13cm}%
    \footnotesize{Note: Number of simulations: 1000, $\lambda = +\infty$. Instruments: $\bG\bX$ if $\bG\by$ is observed, $\hat{\mathbf{G}}\bX$ if $\bG\by$ is not observed and approximated by $\tilde{\mathbf{G}}\by$.}
  \end{minipage}%
}\\
\end{tabular} 

 
\end{table}

\begin{table}[!htbp] 
\centering 
\caption{Simulation results without contextual effects (3).} 
\label{tab:simple3} 
\begin{tabular}{@{\extracolsep{5pt}}ld{4}d{4}d{4}d{4}d{4}} 
\\[-1.8ex]\hline 
\hline \\[-1.8ex] 
Statistic & \multicolumn{1}{c}{Mean} & \multicolumn{1}{c}{Std. Dev.} & \multicolumn{1}{c}{Pctl(25)} & \multicolumn{1}{c}{Median} & \multicolumn{1}{c}{Pctl(75)} \\ 
\hline\hline \\[-1.8ex] 
\multicolumn{6}{c}{$N=50$, $M=100$ - $\mathbf{Gy}$ \textbf{is Observed}}\\\hline \\[-1.8ex] 
\multicolumn{6}{c}{Estimation results}\\\hline\\[-1.8ex] 
$Intercept=2$ & 2.001 & 0.188 & 1.867 & 1.990 & 2.125 \\
$\alpha=0.4$ & 0.400 & 0.010 & 0.393 & 0.401 & 0.407 \\
$\beta_1=1$ & 1.000 & 0.003 & 0.998 & 1.000 & 1.002 \\
$\beta_2=1.5$ & 1.500 & 0.006 & 1.496 & 1.500 & 1.504 \\ \hline\\[-1.8ex] 
\multicolumn{6}{c}{Tests}\\\hline\\[-1.8ex] 
\textit{F}-test & 2776.682 & 416.894 & 2489.415 & 2755.846 & 3036.762 \\
Hausman & 1.673 & 2.285 & 0.157 & 0.756 & 2.307 \\
Sargan & 2.889 & 2.356 & 1.156 & 2.274 & 3.959 \\
 \hline\hline\\[-1.8ex] 
\multicolumn{6}{c}{$N=50$, $M=100$ - $\mathbf{Gy}$ \textbf{is not observed - same draw}}\\\hline\\[-1.8ex] 
\multicolumn{6}{c}{Estimation results}\\\hline\\[-1.8ex] 
$Intercept=2$ & 3.719 & 0.274 & 3.520 & 3.702 & 3.905 \\
$\alpha=0.4$ & 0.306 & 0.015 & 0.296 & 0.307 & 0.316 \\
$\beta_1=1$ & 1.001 & 0.003 & 0.999 & 1.001 & 1.003 \\
$\beta_2=1.5$ & 1.502 & 0.006 & 1.498 & 1.502 & 1.506 \\
\multicolumn{6}{c}{Tests}\\\hline\\[-1.8ex] 
\textit{F}-test & 38566.204 & 5520.495 & 34806.901 & 38162.018 & 42221.999 \\
Hausman & 21.208 & 11.433 & 13.058 & 19.173 & 28.217 \\
Sargan & 247.860 & 32.667 & 225.385 & 246.456 & 268.697 \\
\hline \\[-1.8ex] 
\multicolumn{6}{c}{Validity}\\\hline\\[-1.8ex] 
$cor(\eta_i,\hat{\hat{x}}_{i,1})$ & 0.000 & 0.014 & -0.009 & 0.000 & 0.009 \\
$cor(\eta_i,\hat{\hat{x}}_{i,2})$  & 0.000 & 0.014 & -0.010 & 0.000 & 0.010 \\
\hline\hline\\[-1.8ex] 
\multicolumn{6}{c}{$N=50$, $M=100$ - $\mathbf{Gy}$ \textbf{is not observed - different draws}}\\\hline\\[-1.8ex] 
\multicolumn{6}{c}{Estimation results}\\\hline\\[-1.8ex] 
$Intercept=2$ & 2.002 & 0.202 & 1.857 & 1.999 & 2.137 \\
$\alpha=0.4$ & 0.400 & 0.011 & 0.392 & 0.400 & 0.408 \\
$\beta_1=1$ & 1.000 & 0.003 & 0.998 & 1.000 & 1.002 \\
$\beta_2=1.5$ & 1.500 & 0.006 & 1.496 & 1.500 & 1.504 \\
\hline \\[-1.8ex] 
\multicolumn{6}{c}{Tests}\\\hline\\[-1.8ex] 
\textit{F}-test & 2798.114 & 418.630 & 2508.203 & 2795.093 & 3071.257 \\
Hausman & 218.584 & 34.913 & 192.694 & 217.089 & 240.687 \\
Sargan & 2.828 & 2.232 & 1.112 & 2.293 & 3.888 \\
\hline \\[-1.8ex] 
\multicolumn{6}{c}{Validity}\\\hline\\[-1.8ex] 
$cor(\eta_i,\hat{\hat{x}}_{i,1})$ & 0.000     & 0.014 & -0.009 & 0.000     & 0.009 \\
$cor(\eta_i,\hat{\hat{x}}_{i,2})$& 0.000     & 0.014 & -0.010 & 0.000     & 0.010 \\
\hline \\[-1.8ex]  \\
\multicolumn{6}{l}{%
  \begin{minipage}{13cm}%
    \footnotesize{Note: Number of simulations: 1000, $\lambda = 1$. Instruments: $\left\{(\tilde{\mathbf{G}})^k\bX, k = 1,2 \right\}$.}
  \end{minipage}%
}\\
\end{tabular} 

\end{table}


\begin{table}[!htbp] 
\centering 
\caption{Simulation results without contextual effects.} 
\label{tab:simple4} 
\begin{tabular}{@{\extracolsep{5pt}}ld{4}d{4}d{4}d{4}d{4}} 
\\[-1.8ex]\hline 
\hline \\[-1.8ex] 
Statistic & \multicolumn{1}{c}{Mean} & \multicolumn{1}{c}{Std. Dev.} & \multicolumn{1}{c}{Pctl(25)} & \multicolumn{1}{c}{Median} & \multicolumn{1}{c}{Pctl(75)} \\ 
\hline\hline \\[-1.8ex] 
\multicolumn{6}{c}{$N=50$, $M=100$ - $\mathbf{Gy}$ \textbf{is Observed}}\\\hline \\[-1.8ex] 
\multicolumn{6}{c}{Estimation results}\\\hline\\[-1.8ex] 
$Intercept=2$ & 2.003 & 0.190 & 1.877 & 1.997 & 2.126 \\
$\alpha=0.4$ & 0.400 & 0.010 & 0.393 & 0.400 & 0.407 \\
$\beta_1=1$& 1.000 & 0.003 & 0.998 & 1.000 & 1.002 \\
$\beta_2=1.5$ & 1.500 & 0.006 & 1.496 & 1.500 & 1.504 \\ \hline\\[-1.8ex] 
\multicolumn{6}{c}{Tests}\\\hline\\[-1.8ex] 
\textit{F}-test & 2582.805 & 396.149 & 2310.803 & 2566.537 & 2834.415 \\
Hausman & 1.648 & 2.135 & 0.175 & 0.803 & 2.350 \\
Sargan & 2.962 & 2.547 & 1.153 & 2.313 & 4.007 \\
 \hline\hline\\[-1.8ex] 
\multicolumn{6}{c}{$N=50$, $M=100$ - $\mathbf{Gy}$ \textbf{is not observed - same draw}}\\\hline\\[-1.8ex] 
\multicolumn{6}{c}{Estimation results}\\\hline\\[-1.8ex] 
$Intercept=2$ & 4.088 & 0.312 & 3.885 & 4.068 & 4.283 \\
$\alpha=0.4$ & 0.285 & 0.017 & 0.275 & 0.287 & 0.296 \\
$\beta_1=1$ & 1.001 & 0.003 & 0.999 & 1.001 & 1.004 \\
$\beta_2=1.5$  & 1.502 & 0.007 & 1.498 & 1.502 & 1.507 \\
\multicolumn{6}{c}{Tests}\\\hline\\[-1.8ex] 
\textit{F}-test & 37084.837 & 5430.758 & 33178.701 & 36580.801 & 40451.244 \\
Hausman & 24.804 & 12.850 & 15.008 & 23.435 & 32.737 \\
Sargan & 351.747 & 38.676 & 327.470 & 349.879 & 376.039 \\
\hline \\[-1.8ex] 
\multicolumn{6}{c}{Validity}\\\hline\\[-1.8ex] 
$cor(\eta_i,\hat{\hat{x}}_{i,1})$  & 0.000 & 0.015 & -0.011 & -0.001 & 0.010 \\
$cor(\eta_i,\hat{\hat{x}}_{i,2})$  & 0.000 & 0.014 & -0.010 & 0.000 & 0.010 \\
\hline\hline\\[-1.8ex] 
\multicolumn{6}{c}{$N=50$, $M=100$ - $\mathbf{Gy}$ \textbf{is not observed - different draws}}\\\hline\\[-1.8ex] 
\multicolumn{6}{c}{Estimation results}\\\hline\\[-1.8ex] 
$Intercept=2$ & 2.006 & 0.216 & 1.866 & 2.010 & 2.143 \\
$\alpha=0.4$ & 0.400 & 0.012 & 0.392 & 0.400 & 0.407 \\
$\beta_1=1$ & 1.000 & 0.003 & 0.998 & 1.000 & 1.002 \\
$\beta_2=1.5$  & 1.500 & 0.007 & 1.495 & 1.500 & 1.505 \\
\hline \\[-1.8ex] 
\multicolumn{6}{c}{Tests}\\\hline\\[-1.8ex] 
\textit{F}-test  & 2605.493 & 395.108 & 2339.618 & 2608.021 & 2860.739 \\
Hausman  & 298.171 & 43.582 & 267.427 & 296.419 & 325.031 \\
Sargan & 3.001 & 2.464 & 1.170 & 2.417 & 4.076 \\
\hline \\[-1.8ex] 
\multicolumn{6}{c}{Validity}\\\hline\\[-1.8ex] 
$cor(\eta_i,\hat{\hat{x}}_{i,1})$ & 0.000 & 0.015 & -0.011 & -0.001 & 0.010 \\
$cor(\eta_i,\hat{\hat{x}}_{i,2})$ & 0.000 & 0.014 & -0.010 & 0.000 & 0.010 \\
\hline \\[-1.8ex]  \\
\multicolumn{6}{l}{%
  \begin{minipage}{13cm}%
    \footnotesize{Note: Number of simulations: 1000, $\lambda = +\infty$. Instruments: $\left\{(\tilde{\mathbf{G}})^k\bX, k = 1,2 \right\}$.}
  \end{minipage}%
}\\
\end{tabular} 

\end{table}

\begin{table}[!htbp] 
\centering 
\caption{Simulation results with contextual effects (2).} 
\label{tab:simpleexo2} 
\begin{tabular}{@{\extracolsep{5pt}}ld{4}d{4}d{4}d{4}d{4}} 
\\[-1.8ex]\hline 
\hline \\[-1.8ex] 
Statistic & \multicolumn{1}{c}{Mean} & \multicolumn{1}{c}{Std. Dev.} & \multicolumn{1}{c}{Pctl(25)} & \multicolumn{1}{c}{Median} & \multicolumn{1}{c}{Pctl(75)} \\ 
\hline\hline \\[-1.8ex] 

\multicolumn{6}{c}{$N=50$, $M=100$ - Instrument: $(\tilde{\mathbf{G}})^2\mathbf{X}$ - $\boldsymbol{G}\boldsymbol{y}$ is observed}\\\hline\\[-1.8ex] 
\multicolumn{6}{c}{Estimation results}\\\hline\\[-1.8ex] 
$Intercept=2$ & 2.004 & 0.181 & 1.880 & 2.007 & 2.126 \\
$\alpha=0.4$ & 0.400 & 0.003 & 0.398 & 0.400 & 0.402 \\
$\beta_1=1$  & 1.000 & 0.003 & 0.998 & 1.000 & 1.002 \\
$\beta_2=1.5$  & 1.500 & 0.006 & 1.496 & 1.500 & 1.504 \\
$\gamma_1=5$  & 5.001 & 0.021 & 4.987 & 5.001 & 5.015 \\
$\gamma_2=-3$ & -3.001 & 0.029 & -3.020 & -3.001 & -2.981 \\
 \hline\\[-1.8ex] 
\multicolumn{6}{c}{Tests}\\\hline\\[-1.8ex] 
\textit{F}-test  & 16233.492 & 1898.917 & 14917.312 & 16163.443 & 17491.015 \\
Hausman& 1.239 & 1.768 & 0.102 & 0.504 & 1.627 \\
Sargan & 1.005 & 1.364 & 0.104 & 0.487 & 1.289 \\
\hline\hline\\[-1.8ex] 
\multicolumn{6}{c}{$N=50$, $M=100$ - Instrument: $(\hat{\mathbf{G}})^2\mathbf{X}$ - $\boldsymbol{G}\boldsymbol{y}$ is not observed}\\\hline\\[-1.8ex] 
\multicolumn{6}{c}{Estimation results}\\\hline\\[-1.8ex] 
$Intercept=2$ & 2.002 & 0.217 & 1.855 & 2.005 & 2.150 \\
$\alpha=0.4$ & 0.400 & 0.004 & 0.397 & 0.400 & 0.403 \\
$\beta_1=1$  & 1.000 & 0.003 & 0.998 & 1.000 & 1.002 \\
$\beta_2=1.5$   & 1.500 & 0.006 & 1.496 & 1.500 & 1.504 \\
$\gamma_1=5$ & 5.357 & 0.021 & 5.343 & 5.357 & 5.371 \\
$\gamma_2=-3$ & -2.380 & 0.037 & -2.405 & -2.381 & -2.357 \\
$\hat{\gamma}_1=0$ & -0.356 & 0.024 & -0.372 & -0.356 & -0.340 \\
$\hat{\gamma}_2=0$ & -0.620 & 0.035 & -0.642 & -0.621 & -0.597 \\
\hline \\[-1.8ex] 
\multicolumn{6}{c}{Tests}\\\hline\\[-1.8ex] 
\textit{F}-test & 10741.676 & 1124.978 & 9978.928 & 10687.760 & 11475.206 \\
Hausman& 22.119 & 10.011 & 14.423 & 21.247 & 28.586 \\
Sargan & 0.956 & 1.304 & 0.107 & 0.464 & 1.263 \\
\hline \\[-1.8ex]  \\
\multicolumn{6}{l}{%
  \begin{minipage}{13cm}%
    \footnotesize{Note: Number of simulations: 1000, $\lambda = +\infty$.}
  \end{minipage}%
}\\
\end{tabular}

\end{table}



\begin{table}[!htbp] 
\centering 
\caption{Simulation results with subpopulation unobserved fixed effects.} 
\label{tab:simpleFE1} 
\begin{tabular}{@{\extracolsep{5pt}}ld{4}d{4}d{4}d{4}d{4}} 
\\[-1.8ex]\hline 
\hline \\[-1.8ex] 
Statistic & \multicolumn{1}{c}{Mean} & \multicolumn{1}{c}{Std. Dev.} & \multicolumn{1}{c}{Pctl(25)} & \multicolumn{1}{c}{Median} & \multicolumn{1}{c}{Pctl(75)} \\ 
\hline\hline \\[-1.8ex] 

\multicolumn{6}{c}{$N=50$, $M=100$ - Instrument: $\mathbf{J}(\tilde{\mathbf{G}})^2\mathbf{X}$ - $\hat{\mathbf{y}}$ is observed}\\\hline\\[-1.8ex] 
\multicolumn{6}{c}{Estimation results}\\\hline\\[-1.8ex]
$\alpha=0.4$ & 0.379 & 1.703 & -0.122 & 0.398 & 0.938 \\
$\beta_1=1$& 1.000 & 0.005 & 0.997 & 1.000 & 1.003 \\
$\beta_2=1.5$ & 1.500 & 0.009 & 1.496 & 1.500 & 1.505 \\
$\gamma_1=5$ & 5.018 & 1.318 & 4.584 & 5.001 & 5.415 \\
& 4.970 & 1.372 & 4.565 & 4.992 & 5.421 \\ 
$\gamma_2=-3$ & -2.967 & 2.710 & -3.861 & -2.998 & -2.156 \\
\hline \\[-1.8ex] 
\multicolumn{6}{c}{Tests}\\\hline\\[-1.8ex] 
\textit{F}-test& 2.860 & 2.270 & 1.132 & 2.364 & 4.045 \\
Hausman & 1.029 & 1.398 & 0.105 & 0.484 & 1.392 \\
Sargan & 0.820 & 1.184 & 0.066 & 0.335 & 1.078 \\
\hline\hline \\[-1.8ex] 
\multicolumn{6}{c}{$N=50$, $M=100$ - Instrument: $\mathbf{J}(\hat{\mathbf{G}})^2\mathbf{X}$ - $\hat{\mathbf{y}}$ is not observed}\\\hline\\[-1.8ex] 
\multicolumn{6}{c}{Estimation results}\\\hline\\[-1.8ex] 
$\alpha=0.4$ & 0.345 & 1.609 & -0.246 & 0.265 & 0.869 \\
$\beta_1=1$ & 1.000 & 0.005 & 0.997 & 1.000 & 1.002 \\
$\beta_2=1.5$& 1.500 & 0.008 & 1.495 & 1.500 & 1.505 \\
$\gamma_1=5$  & 5.351 & 0.170 & 5.284 & 5.343 & 5.408 \\
$\gamma_2=-3$ & -2.378 & 0.123 & -2.416 & -2.373 & -2.331 \\
$\hat{\gamma}_1=0$ & -0.307 & 1.442 & -0.769 & -0.236 & 0.237 \\
$\hat{\gamma}_2=0$ & -0.534 & 2.490 & -1.346 & -0.407 & 0.398 \\
\hline \\[-1.8ex] 
\multicolumn{6}{c}{Tests}\\\hline\\[-1.8ex]
\textit{F}-test & 2.773 & 2.189 & 1.072 & 2.304 & 3.773 \\
Hausman & 1.114 & 1.563 & 0.105 & 0.525 & 1.483 \\
Sargan & 0.889 & 1.329 & 0.083 & 0.381 & 1.206 \\
\hline \\[-1.8ex]  \\
\multicolumn{6}{l}{%
  \begin{minipage}{11cm}%
    \footnotesize{Note: Number of simulations: 1000, $\lambda = 1$. In each group, the fixed effect is generated as $0.3x_{1,1} + 0.3x_{3,2} - 1.8x_{50,2}$.}
  \end{minipage}%
}\\
\end{tabular}
\end{table}

\begin{table}[!htbp] 
\centering 
\caption{Simulation results with subpopulation unobserved fixed effects (2).} 
\label{tab:simpleFE2} 
\begin{tabular}{@{\extracolsep{5pt}}ld{4}d{4}d{4}d{4}d{4}} 
\\[-1.8ex]\hline 
\hline \\[-1.8ex] 
Statistic & \multicolumn{1}{c}{Mean} & \multicolumn{1}{c}{Std. Dev.} & \multicolumn{1}{c}{Pctl(25)} & \multicolumn{1}{c}{Median} & \multicolumn{1}{c}{Pctl(75)} \\ 
\hline\hline \\[-1.8ex] 

\multicolumn{6}{c}{$N=50$, $M=100$ - Instrument: $\mathbf{J}(\tilde{\mathbf{G}})^2\mathbf{X}$ - $\hat{\mathbf{y}}$ is observed}\\\hline\\[-1.8ex] 
\multicolumn{6}{c}{Estimation results}\\\hline\\[-1.8ex]
$\alpha=0.4$& 0.623 & 4.670 & -0.475 & 0.341 & 1.345 \\
$\beta_1=1$& 1.001 & 0.015 & 0.997 & 1.000 & 1.003 \\
$\beta_2=1.5$& 1.499 & 0.019 & 1.494 & 1.500 & 1.504 \\
$\gamma_1=5$ & 4.826 & 3.644 & 4.263 & 5.042 & 5.688 \\
$\gamma_2=-3$ & -3.357 & 7.485 & -4.491 & -2.913 & -1.572 \\
\hline \\[-1.8ex] 
\multicolumn{6}{c}{Tests}\\\hline\\[-1.8ex] 
\textit{F}-test & 1.025 & 1.023 & 0.293 & 0.710 & 1.451 \\
Hausman & 0.979 & 1.527 & 0.090 & 0.396 & 1.264 \\
Sargan & 0.665 & 1.184 & 0.042 & 0.203 & 0.801 \\

\hline\hline \\[-1.8ex] 
\multicolumn{6}{c}{$N=50$, $M=100$ - Instrument: $\mathbf{J}(\hat{\mathbf{G}})^2\mathbf{X}$ - $\hat{\mathbf{y}}$ is not observed}\\\hline\\[-1.8ex] 
\multicolumn{6}{c}{Estimation results}\\\hline\\[-1.8ex] 
$\alpha=0.4$ & -0.071 & 3.561 & -0.949 & -0.047 & 0.876 \\
$\beta_1=1$ & 0.999 & 0.010 & 0.996 & 0.999 & 1.002 \\
$\beta_2=1.5$ & 1.500 & 0.018 & 1.495 & 1.501 & 1.506 \\
$\gamma_1=5$  & 5.305 & 0.377 & 5.208 & 5.306 & 5.406 \\
$\gamma_2=-3$  & -2.364 & 0.192 & -2.411 & -2.355 & -2.306 \\
$\hat{\gamma}_1=0$ & 0.062 & 3.183 & -0.777 & 0.051 & 0.846 \\
$\hat{\gamma}_2=0$ & 0.117 & 5.512 & -1.360 & 0.062 & 1.459 \\
\hline \\[-1.8ex] 
\multicolumn{6}{c}{Tests}\\\hline\\[-1.8ex]
\textit{F}-test & 1.063 & 1.046 & 0.329 & 0.741 & 1.486 \\
Hausman & 0.993 & 1.499 & 0.095 & 0.409 & 1.255 \\
Sargan & 0.670 & 1.117 & 0.041 & 0.207 & 0.817 \\
\hline \\[-1.8ex] \\
\multicolumn{6}{l}{%
  \begin{minipage}{11cm}%
    \footnotesize{Note: Number of simulations: 1000, $\lambda = +\infty$. In each group, the fixed effect is generated as $0.3x_{1,1} + 0.3x_{3,2} - 1.8x_{50,2}$.}
  \end{minipage}%
}\\
\end{tabular}
\end{table}


\begin{table}[!htbp] 
\centering 
\caption{Simulation results with ARD: without contextual effects (1000 replications).} 
\label{tab:ARD_gamma0} 
\begin{tabular}{@{\extracolsep{5pt}}ld{4}d{4}d{4}d{4}d{4}} 
\\[-1.8ex]\hline 
\hline \\[-1.8ex] 
Statistic & \multicolumn{1}{c}{Mean} & \multicolumn{1}{c}{Std. Dev.} & \multicolumn{1}{c}{Pctl(25)} & \multicolumn{1}{c}{Median} & \multicolumn{1}{c}{Pctl(75)} \\ 
\hline\hline \\[-1.8ex] 

\multicolumn{6}{c}{$N=250$, $M=20$ - Instrument: $\tilde{\mathbf{G}}\mathbf{X}$ - $\bG\by$ is observed}\\\hline\\[-1.8ex] 
\multicolumn{6}{c}{Estimation results}\\\hline\\[-1.8ex]
$Intercept=2$ & 2.031 & 0.941 & 1.471 & 2.048 & 2.608 \\ 
$\alpha=0.4$ & 0.398 & 0.051 & 0.368 & 0.397 & 0.429 \\ 
$\beta_1=1$ & 1.000 & 0.003 & 0.998 & 1.000 & 1.002 \\ 
$\beta_2=1.5$ & 1.500 & 0.006 & 1.496 & 1.500 & 1.504 \\ 
\hline \\[-1.8ex] 
\multicolumn{6}{c}{Tests}\\\hline\\[-1.8ex] 
\textit{F}-test & 152.722 & 63.626 & 104.971 & 145.232 & 189.435 \\ 
Hausman & 1.037 & 1.467 & 0.098 & 0.435 & 1.352 \\ 
Sargan & 1.003 & 1.407 & 0.096 & 0.422 & 1.335 \\ 
\hline\hline \\[-1.8ex] 
\multicolumn{6}{c}{$N=250$, $M=20$ - Instrument: $\left\{\left(\tilde{\mathbf{G}}\right)^k\mathbf{X}, k = 1, 2\right\}$ -$\bG\by$ is observed}\\\hline\\[-1.8ex] 
\multicolumn{6}{c}{Estimation results}\\\hline\\[-1.8ex] 
$Intercept=2$ & 1.999 & 0.429 & 1.721 & 1.985 & 2.254 \\ 
$\alpha=0.4$ & 0.400 & 0.023 & 0.386 & 0.400 & 0.415 \\ 
$\beta_1=1$ & 1.000 & 0.003 & 0.998 & 1.000 & 1.002 \\ 
$\beta_2=1.5$ & 1.500 & 0.006 & 1.496 & 1.500 & 1.504 \\ 
\hline \\[-1.8ex] 
\multicolumn{6}{c}{Tests}\\\hline\\[-1.8ex] 
\textit{F}-test & 427.225 & 146.605 & 319.567 & 417.901 & 517.949 \\ 
Hausman & 1.026 & 1.467 & 0.116 & 0.491 & 1.339 \\ 
Sargan & 3.000 & 2.442 & 1.218 & 2.342 & 4.089 \\ 
\hline\hline \\[-1.8ex] 
\multicolumn{6}{c}{$N=250$, $M=20$ - Instrument: $\hat{\mathbf{G}}\mathbf{X}$ - $\bG\by$ is not observed}\\\hline\\[-1.8ex] 
\multicolumn{6}{c}{Estimation results}\\\hline\\[-1.8ex]
$Intercept=2$ & 1.854 & 1.117 & 1.182 & 1.879 & 2.569 \\
$\alpha=0.4$ & 0.408 & 0.061 & 0.368 & 0.407 & 0.445 \\ 
$\beta_1=1$ & 1.000 & 0.003 & 0.998 & 1.000 & 1.002 \\ 
$\beta_2=1.5$ & 1.500 & 0.007 & 1.496 & 1.500 & 1.505 \\ 
\hline \\[-1.8ex] 
\multicolumn{6}{c}{Tests}\\\hline\\[-1.8ex] 
\textit{F}-test & 144.813 & 60.270 & 100.244 & 138.238 & 178.694 \\ 
Hausman & 30.339 & 14.849 & 19.275 & 27.985 & 39.404 \\ 
Sargan & 1.105 & 1.576 & 0.109 & 0.506 & 1.450 \\ 
\hline\hline \\[-1.8ex] 
\multicolumn{6}{c}{$N=250$, $M=20$ - Instrument: $\left\{\left(\hat{\mathbf{G}}\right)^k\mathbf{X}, k = 1, 2\right\}$ - $\bG\by$ is not observed}\\\hline\\[-1.8ex] 
\multicolumn{6}{c}{Estimation results}\\\hline\\[-1.8ex] 
$Intercept=2$ & 1.969 & 0.531 & 1.599 & 1.962 & 2.318 \\ 
$\alpha=0.4$ & 0.402 & 0.029 & 0.383 & 0.402 & 0.422 \\ 
$\beta_1=1$ & 1.000 & 0.003 & 0.998 & 1.000 & 1.002 \\ 
$\beta_2=1.5$ & 1.500 & 0.007 & 1.496 & 1.500 & 1.505 \\ 
\hline \\[-1.8ex] 
\multicolumn{6}{c}{Tests}\\\hline\\[-1.8ex] 
\textit{F}-test & 419.464 & 142.058 & 314.376 & 407.311 & 505.246 \\ 
Hausman & 171.162 & 53.370 & 133.847 & 169.651 & 205.461 \\ 
Sargan & 3.274 & 2.575 & 1.346 & 2.613 & 4.443 \\ 
\hline\hline \\[-1.8ex] 
\end{tabular}
\end{table}


\begin{table}[htbp]
\centering 
\caption{Simulation results with nuclear ARD: without contextual effects, and $\hat{\by}$ is observed (1000 replications).} 
\label{tab:nuclear_gamma0} 
    \begin{tabular}{@{\extracolsep{5pt}}lld{4}d{4}d{4}d{4}d{4}}
\\[-1.8ex]\hline 
\hline \\[-1.8ex] 
\multicolumn{2}{l}{Weight$^\dagger$} & \multicolumn{1}{c}{Mean} & \multicolumn{1}{c}{Std. Dev.} & \multicolumn{1}{c}{Pctl(25)} & \multicolumn{1}{c}{Median} & \multicolumn{1}{c}{Pctl(75)} \\ 
\hline\hline \\[-1.8ex] 

\multicolumn{7}{c}{$N=250$, $M=20$ - Instrument: $\tilde{\mathbf{G}}\mathbf{X}$ - $\bG\by$ is observed}\\\hline\\[-1.8ex] 
   $\tau =$ 200   &   $\alpha=0.4$    & 0.403  &  0.088  &0.350  &0.406 & 0.456\\
   $\tau =$ 600   &   $\alpha=0.4$    & 0.396  &  0.139  &0.322  &0.396 & 0.468 \\
   $\tau =$ 1374  &   $\alpha=0.4$    &  0.399 &0.242 & 0.279 &0.396  & 0.516\\
\hline\hline \\[-1.8ex] 
\multicolumn{7}{c}{$N=250$, $M=20$ - Instrument: $\left\{\left(\hat{\mathbf{G}}\right)^k\mathbf{X}, k = 1, 2\right\}$ - $\bG\by$ is observed}\\\hline\\[-1.8ex] 
   $\tau =$ 200   &  $\alpha=0.4$     & 0.400  &  0.036  &0.378&  0.401  &0.422\\
   $\tau =$ 600   &   $\alpha=0.4$    & 0.396 &0.050  &0.368  &0.398 & 0.427 \\
   $\tau =$ 1374  &   $\alpha=0.4$    & 0.403  &  0.111 &    0.346 &    0.402 &    0.461\\
\hline\hline \\[-1.8ex] \\
\multicolumn{7}{l}{%
  \begin{minipage}{11.6cm}%
    \footnotesize{Note: The parameter $\tau$ corresponds to the parameter $\lambda$ in \cite{alidaee2020recovering} and represents the weight associated to the nuclear norm. In our context, the recommended value of \cite{alidaee2020recovering} is given by $\tau=1374$. The optimal value (in terms of RMSE) found through cross-validation is $\tau=600$, while $\tau=200$ gives a RMSE similar to the recommended value.}
  \end{minipage}%
}\\
    \end{tabular}%
    
\end{table}%


\begin{table}[htbp]
\centering 
\caption{Simulation results with nuclear ARD: $\hat{\by}$ is observed, $\tau=600$ (1000 replications).} 
\label{tab:ARD_gammadif0:gyobs} 
\begin{tabular}{@{\extracolsep{5pt}}ld{4}d{4}d{4}d{4}d{4}} 
\\[-1.8ex]\hline 
\hline \\[-1.8ex] 
Statistic & \multicolumn{1}{c}{Mean} & \multicolumn{1}{c}{Std. Dev.} & \multicolumn{1}{c}{Pctl(25)} & \multicolumn{1}{c}{Median} & \multicolumn{1}{c}{Pctl(75)} \\ 
\hline\hline \\[-1.8ex] 

\multicolumn{6}{c}{$N=250$, $M=20$ - Instrument: $\tilde{\mathbf{G}}\mathbf{X}^2$ - $\bG\by$ is observed}\\\hline\\[-1.8ex] 
\multicolumn{6}{c}{Estimation results}\\\hline\\[-1.8ex]
$Intercept=2$ & 2.001 & 0.267 & 1.825 & 1.999 & 2.181 \\ 
$\alpha=0.4$ & 0.400 & 0.011 & 0.393 & 0.400 & 0.406 \\ 
$\beta_1=1$ & 1.000 & 0.003 & 0.998 & 1.000 & 1.002 \\ 
$\beta_2=1.5$ & 1.500 & 0.006 & 1.496 & 1.500 & 1.504 \\ 
$\gamma_1=5$ & 5.001 & 0.027 & 4.982 & 5.001 & 5.020 \\ 
$\gamma_2=-3$ & -3.000 & 0.033 & -3.022 & -2.999 & -2.977 \\ 
\hline\\[-1.8ex] 
\multicolumn{6}{c}{Tests}\\\hline\\[-1.8ex] 
\textit{F}-test  & 810.356 & 338.648 & 570.099 & 774.973 & 1005.605 \\ 
Hausman  & 0.956 & 1.281 & 0.113 & 0.467 & 1.310 \\ 
Sargan & 1.033 & 1.417 & 0.107 & 0.515 & 1.395 \\ 
\hline\hline \\[-1.8ex]
    \end{tabular}%
\end{table}%



\begin{table}[htbp]
\centering 
\caption{Simulation results with nuclear ARD: $\hat{\by}$ is not observed, $\tau=600$ (1000 replications).} 
\label{tab:ARD_gammadif0:gynoobs} 
\begin{tabular}{@{\extracolsep{5pt}}ld{4}d{4}d{4}d{4}d{4}} 
\\[-1.8ex]\hline 
\hline \\[-1.8ex] 
Statistic & \multicolumn{1}{c}{Mean} & \multicolumn{1}{c}{Std. Dev.} & \multicolumn{1}{c}{Pctl(25)} & \multicolumn{1}{c}{Median} & \multicolumn{1}{c}{Pctl(75)} \\ 
\hline\hline \\[-1.8ex] 

\multicolumn{6}{c}{$N=250$, $M=20$ - Instrument: $\tilde{\mathbf{G}}\mathbf{X}$ - $\bG\by$ is not observed}\\\hline\\[-1.8ex] 
\multicolumn{6}{c}{Estimation results}\\\hline\\[-1.8ex]
$Intercept=2$ & 5.215 & 2.934 & 4.008 & 5.423 & 6.748 \\
$\alpha=0.4$ & 0.225 & 0.161 & 0.141 & 0.214 & 0.291 \\ 
$\beta_1=1$ & 1.001 & 0.004 & 0.998 & 1.001 & 1.003 \\ 
$\beta_2=1.5$ & 1.501 & 0.007 & 1.497 & 1.501 & 1.505 \\ 
\hline\\[-1.8ex] 
\multicolumn{6}{c}{Tests}\\\hline\\[-1.8ex] 
\textit{F}-test & 21.033 & 13.187 & 11.490 & 18.861 & 28.535 \\ 
Hausman & 7.626 & 6.980 & 2.377 & 5.937 & 10.976 \\ 
Sargan & 2.488 & 3.432 & 0.258 & 1.191 & 3.313 \\ 
$cor(\eta_i,\hat{x}_{i,1})$ & -0.006 & 0.022 & -0.020 & -0.006 & 0.008 \\ 
$cor(\eta_i,\hat{x}_{i,2})$ & -0.036 & 0.029 & -0.055 & -0.036 & -0.016 \\ 
\hline\hline \\[-1.8ex] 
\multicolumn{6}{c}{$N=250$, $M=20$ - Instrument: $\left\{\left(\hat{\mathbf{G}}\right)^k\mathbf{X}, k = 1, 2\right\}$ - $\bG\by$ is not observed}\\\hline\\[-1.8ex] 
\multicolumn{6}{c}{Estimation results}\\\hline\\[-1.8ex] 
$Intercept=2$ & 4.481 & 1.503 & 3.469 & 4.493 & 5.474 \\ 
$\alpha=0.4$ & 0.266 & 0.082 & 0.211 & 0.264 & 0.321 \\ 
$\beta_1=1$ & 1.001 & 0.004 & 0.998 & 1.001 & 1.003 \\ 
$\beta_2=1.5$ & 1.501 & 0.007 & 1.496 & 1.501 & 1.506 \\ 
\hline\\[-1.8ex] 
\multicolumn{6}{c}{Tests}\\\hline\\[-1.8ex] 
\textit{F}-test & 50.332 & 24.549 & 31.909 & 46.716 & 64.013 \\ 
Hausman & 57.141 & 40.279 & 27.257 & 48.421 & 79.545 \\ 
Sargan & 11.075 & 9.786 & 4.209 & 7.877 & 15.298 \\ 
$cor(\eta_i,\hat{\hat{x}}_{i,1})$ & -0.011 & 0.023 & -0.025 & -0.011 & 0.005 \\ 
$cor(\eta_i,\hat{\hat{x}}_{i,2})$ & -0.064 & 0.040 & -0.092 & -0.064 & -0.036 \\ 
\hline\hline \\[-1.8ex]
    \end{tabular}%
\end{table}%


\cleardoublepage




\newpage
\subsection{Expectation Maximization Algorithm}\label{sec:EM}

If $\mathbf{A}$ was observed, the objective would be to maximize the log-likelihood of the model with respect to $\boldsymbol{\theta}$:
$$
\mathcal{P}(\mathbf{y}|\mathbf{A},\mathbf{X};\boldsymbol{\theta}).
$$
Since $\mathbf{A}$ is unobserved, we propose to treat it as a latent variable. We therefore look for the value of $\boldsymbol{\theta}$ that maximizes:
$$
\mathcal{P}(\mathbf{y}|\mathbf{X};\boldsymbol{\theta})=\sum_\mathbf{A} \mathcal{P}(\mathbf{y}|\mathbf{A},\mathbf{X};\boldsymbol{\theta})P(\mathbf{A}).
$$
Since the number potential network structures is huge, evaluating this expectation is unfeasible.\footnote{For a population of only 5 individuals, the number of network structures is $2^{20}$.} We therefore propose to maximize $\mathcal{P}(\mathbf{y}|\mathbf{X};\boldsymbol{\theta})$ using an expectation maximization algorithm:
\begin{algorithm}\label{algo:EM} Initialize $\boldsymbol{\theta}_0$, and for $t=0,...,T$, do the following:
\begin{enumerate}
    \item Use a Metropolis--Hastings algorithm (see Algorithm \ref{algo:mcmc}) to obtain the draws $(\mathbf{A}_1,...,\mathbf{A}_R)$ from $P(\mathbf{A}|\mathbf{y},\boldsymbol{\theta}_t)$.
    \item Evaluate $$Q_t(\boldsymbol{\theta})\approx \sum_{r=1}^{R}\mathcal{P}(\mathbf{y}|\mathbf{A}_r,\mathbf{X};\boldsymbol{\theta}_t).$$
    \item Set $\boldsymbol{\theta}_{t+1}=\arg\max Q_t(\boldsymbol{\theta}).$
\end{enumerate}
\end{algorithm}
